# Supplementary material for: Evaluation of Human Visual Privacy Protection: A Three-Dimensional Framework and Benchmark Dataset
Source: arXiv:2507.13981 source file (2025-07-18)
Supplement: Supplementary file 1 [file 7_appendix.tex]

\setcounter{equation}{0}
\setcounter{figure}{0}
\setcounter{table}{0}
\setcounter{page}{1}
\makeatletter

 % This line requires natbib
 % This line requires natbib

\title{Supplementary Material}
Fig. \ref{fig:HR-VISPR-object-distribution} shows the distribution of these labels in HR-VISPR. The remaining COCO labels are highly irrelevant to this study and are rarely present in HR-VISPR.

\begin{figure}
    \centering
    \includegraphics[width=\linewidth]{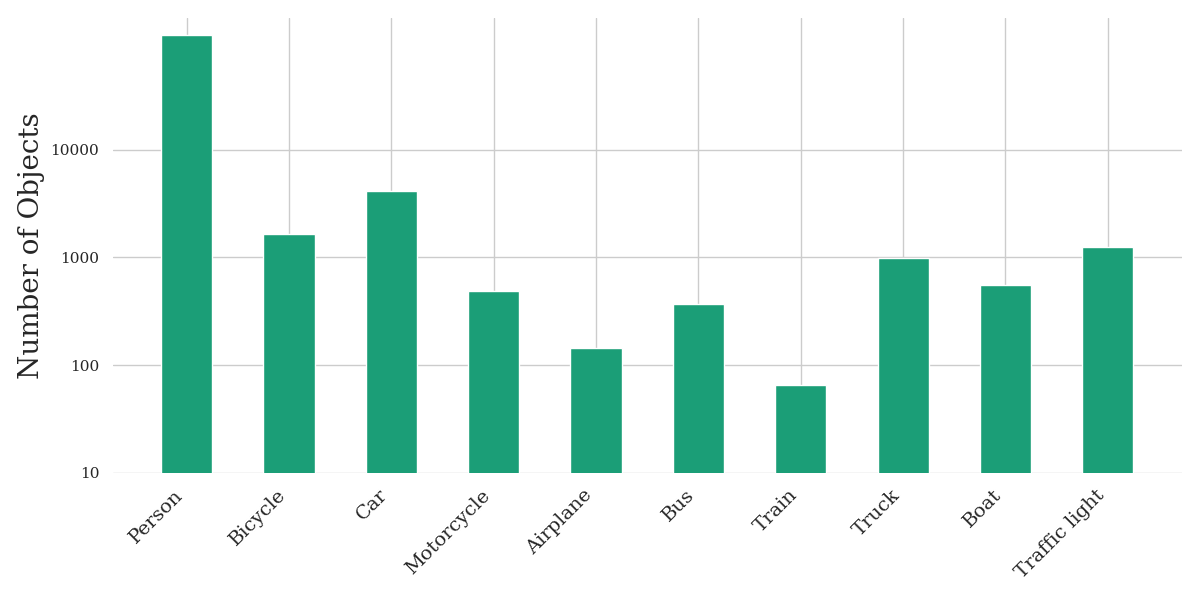}
    \caption{Object label distribution in the HR-VISPR dataset. The vertical axis represents the number of object instances per object class. }
    \label{fig:HR-VISPR-object-distribution}
\end{figure}

\begin{figure}
    \centering
    \includegraphics[width=\linewidth]{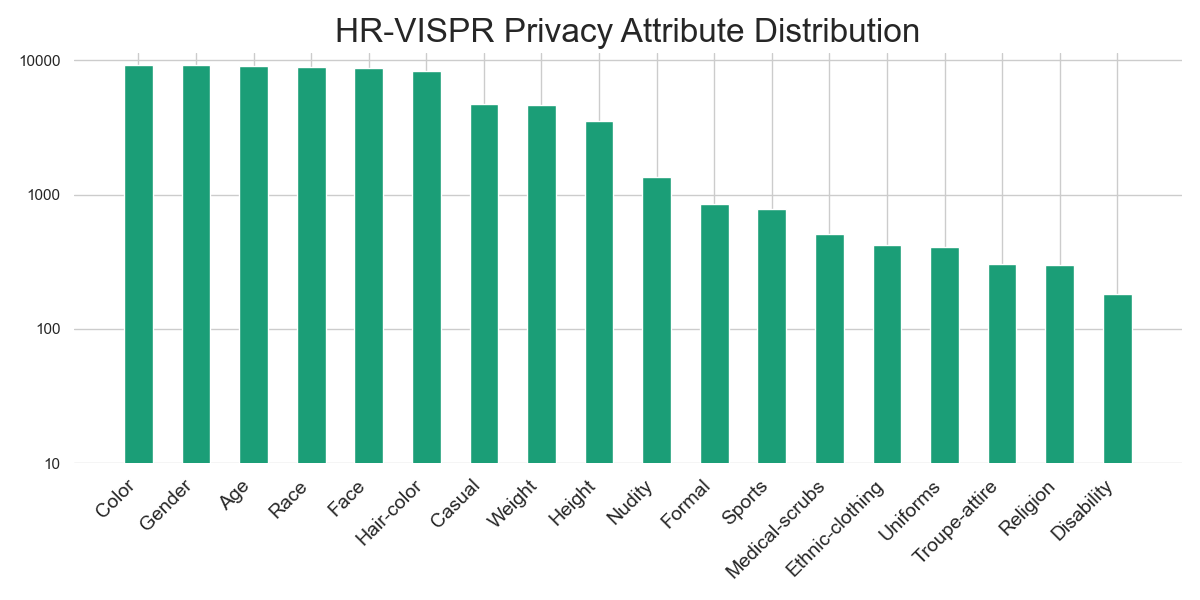}
    \caption{Label distribution in the HR-VISPR dataset. The vertical axis represents the number of images per attribute. }
    \label{fig:HR-VISPR-distribution}
\end{figure}

Fig. \ref{fig:auc} summarizes the utility results, presenting the average Area Under PR Curves (AUC) across classes for each method. Clearly, the HS and HE show the highest utility performance, followed by HM, H2D, H3D, HP, and HB. Although this analysis highlights utility differences across anonymization methods, identifying the exact causes of utility model failures remains challenging. Certain anonymization techniques introduce additional noise due to poor human segmentation, missed detections, and occlusions involving humans and other objects. Additionally, the introduction of unique features, such as blurred regions, avatars, embossing effects (highlight and shadow), or encrypted pixels, may introduce bias to the models. For these reasons, it can be difficult to draw generalized conclusions from these results to other tasks and contexts with different datasets. Nevertheless, applying the same evaluation framework and procedure to these tasks offers a structured approach to extracting the same trade-off insights.

\begin{figure}
    \centering
    \includegraphics[width=0.5\textwidth]{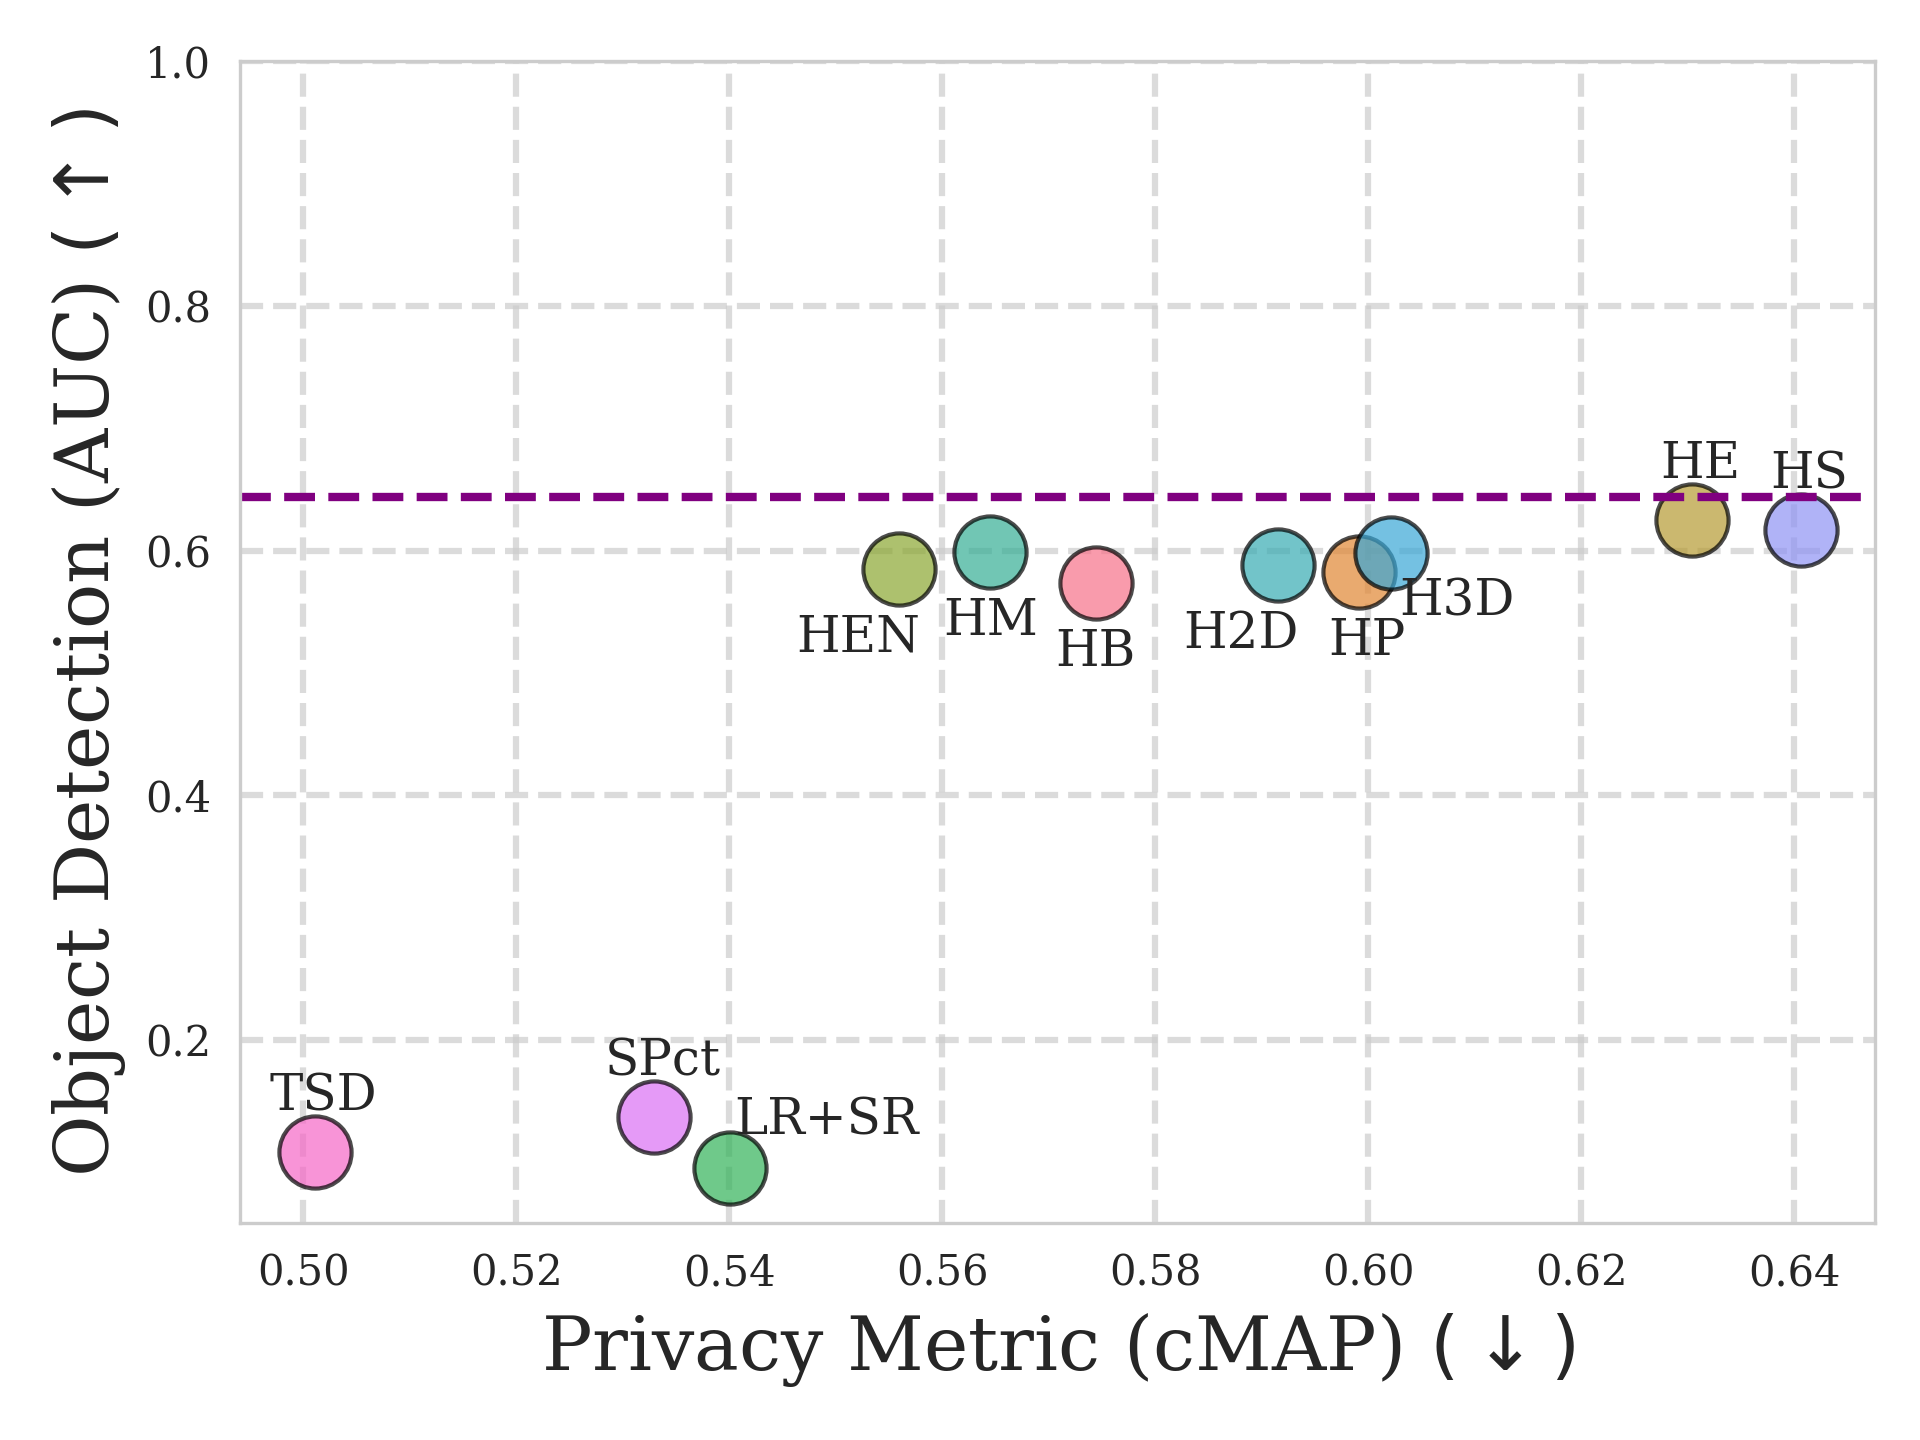}
    \caption{The privacy-utility trade-off evaluation for the anonymization methods, with utility represented as the average AUC of all HR-VISRP object. }
    \label{fig:auc}
\end{figure}

\setlength\tabcolsep{1pt}
\begin{table}[hbtp!]
    \caption{Implementation details and notation of the anonymization methods selected for the trade-off analysis. } \label{tab:implemented-methods}
     \begin{center}
     \resizebox{\columnwidth}{!}{%
    \begin{tabular}{@{}p{3cm}p{1.5cm}p{1.5cm}p{8cm}@{}}

        % \Xhline{1pt}
        \toprule
        Methods
        & Papers
        & Notation 
        & Implementation Details
        \\ 
        \midrule

         Human Blurring
         & \cite{82_tay2024privobfnet,HAR16_zhang2021multi}%,AD4_cucchiara2024video}             
         & HB
         & Seg. \cite{segmentor}, followed by blurring $(k=101)$\footnotemark[1]
         \\

         Human Pixelation 
         & \cite{35_climent2021protection}
         &HP
         & Seg. \cite{segmentor}, followed by pixelation $(k=20)$ %\footnotemark[1]
         \\
         
         Human Embossing 
         & \cite{35_climent2021protection}
         &  HE 
         & Seg. \cite{segmentor}, followed by embossing $(k=3)$ %\footnotemark[1] 
         \\

         Human Masking
         &\cite{AD5_yan2020image}  
         &HM
         &Seg. \cite{segmentor}, followed by blackening %\footnotemark[1]
         \\
         
         Human Encryption
         & \cite{14_shifa2020skin}
         &  HEN
         & Seg. \cite{segmentor}, followed by AES pixel Encryption %\footnotemark[1]  
         \\

         Human 2D Avatars 
         & \cite{35_climent2021protection}
         & H2D 
         & DensePose \cite{DensePose} with customized avatar
         \\

         Human 3D Avatar
         &\cite{51_shen2023privacy,17_sattar2020body}
         & H3D 
         & ROMP \cite{ROMP} 
         \\

         Human Synthesis
         &\cite{72_hukkelaas2023deepprivacy2}
         & HS
         & DeepPrivacy2 \cite{72_hukkelaas2023deepprivacy2} 
         \\

          Low Resolution + Super Resolution 
          & \cite{99_hou2021extreme}
          & LR+SR
          & \makecell[tl]{Downscale (30×30) \cite{HAR40_wang2023modeling}, upscale by SR (×8) \cite{LapSRN}, \\followed by SR (×3) \cite{FSRCNN}}
         \\

         SPAct
        & \cite{HAR30_dave2022spact}
        & SPct
        & Public Implementation
        \\
        
        TeD-SPAD
        &\cite{AD10_fioresi2023ted} 
        &TSD
        & Public Implementation
        \\
        \bottomrule
        
    \end{tabular}
    }
    \end{center}
\end{table}

% ////////////////////////////////////////////////////////
+++++++++++++++++++ talk about the augmentation 
For training of the privacy classifier, the dataset was augmented similarly to prior works \cite{VISPR, AD10_fioresi2023ted,HAR30_dave2022spact,HAR3_wu2020privacy}. Additionally, we applied random shifting, scaling, rotation, transpose, grid-distortion, and elastic-transform from Albumentation library \cite{buslaev2020albumentations}.
% For training of the utility model, the same training, validation, and testing sets are used. 
% We applied the default augmentation techniques provided in the YOLOv11 framework \cite{yolov8}. 
% The HR-VISPR dataset, along with its anonymized versions and corresponding privacy and utility labels, is publicly available.  

\subsection{Metrics Implementation} \label{sec:implementation-details}
 Details about the privacy, utility, and practicality metric implementation are provided in \textcolor{red}{Appendix[]} 
\subsubsection{Privacy Metric} \label{exp:privacy-metric-training} A ResNet50 backbone was adopted for the multi-label classifier. The model was trained on the HR-VISPR at a 224 × 224 resolution for 100 epochs. The starting learning rate was $1e-3$, following a linear warmup and a scheduler that drops 1/5 with loss stagnation \cite{AD10_fioresi2023ted}, \cite{HAR30_dave2022spact}. The batch size was set to 32, and we used Adam optimizer. To compensate for the class imbalance in this multi-label classification setup, we applied class-wise loss weighting ($W_c$), where weights are inversely proportional to class frequency and normalized by the number of classes. The weights are computed as \( W_c = \frac{N}{N_c \times C} \), where \( N \), \( N_c \), and \( C \) denote the total number of samples, the number of samples per class, and the total number of classes, respectively.

% The weights are obtained with the equation

% \begin{equation}
% W_c = \frac{N}{N_c \times C} , \label{eq:wc} 
% \end{equation} 

% where \textit{N, $N_c$,} and \textit{C} are the total number of samples, the number of samples per class, and the number of classes, respectively. 

\subsubsection{Utility Metric} A YOLOv11 detector \cite{yolov8} was trained, following the same training strategy presented by the authors, on the 11 anonymized versions of HR-VISPR. For evaluation, the precision, F1-score, and AUC scores are computed for each anonymized version.

\subsubsection{Practicality Metric}
\noindent \textbf{Throughput Score.} We measured throughput in a unified setting to eliminate variations due to image size and computational power reported in previous works. First, we selected 40 images from HR-VISPR containing multiple human instances. The images were then resized into $640 \times 640$ and processed by all anonymization methods, on a gpu-enabled RTX 4090 device, to compute the throughput according to Eq.\ref{eq:fps}. The processing time includes both the detection and anonymization time. 

\noindent \textbf{Robustness Score} We applied human detection on anonymized images, similarly to utility, but employing a pre-trained model \cite{yolov8}. First, human objects were detected on the anonymized and original test sets of the HR-VISPR. Then, detections in the original and anonymized sets were matched based on IoU and SSIM scores. Since background details are visible within human-object bounding boxes, we applied a 0.99 threshold to prevent matches driven by background similarity alone. Instances with similarity scores higher than the threshold are summed up, representing the method's robustness score. 

\noindent \textbf{Intelligibility Score} We computed the CMMD metric \cite{CMMD} between the original and anonymized HR-VISPR test sets. Since CMMD quantifies discrepancy, lower values indicate a higher similarity to the original data, corresponding to a higher intelligibility.  

The three scores are combined as detailed in the previous section. To ensure comparability, the inverted robustness and intelligibility scores were normalized (min-max scaling) before integration into the practicality score. 
To further demonstrate the effect of anonymization methods on utility, we analyze the Precision-Recall (PR) curves for the different classes under each anonymization method, as shown in Fig. \ref{fig:pr_curves}. The analysis reveals that the approaches which show similar anonymization effects, according to the human perception, may differ in their influence on utility. For instance, although both HM and HEN fully remove human figures, their utility performance varies significantly. HEN consistently underperforms HM (person, bicycle, car, airplane, bus, truck, and boat), suggesting that the noisy masks in HEN disrupt the utility more than the single-color masks HM. In contrast, HP and HB tend to align in most cases despite their different anonymization effects, except that HP shows better performance on few (non-human) classes, such as bus and truck. Despite revealing fine human features in the highlight and shadow effects, HE does not contribute to a higher utility compared to HM, HEN, HP, and HB, except for the person class, suggesting a reinforcement of model bias towards human detection. H2D and H3D reveal human parts in virtual avatars, and are mostly correlated in performance, except for few objects, such as person, motorcycle, and bicycle, where H2D is superior to H3D. This is likely due to the misalignment between human figures and avatars in H3D, which introduces significant noise into the data. %This is highly likely attributed to the imprecise human-to-avatar alignment in H3D, which introduces significant noise to the data. 

\begin{figure*}[!hptb]
\centering
\subfloat[all classes]{ \includegraphics[width=0.35\linewidth]{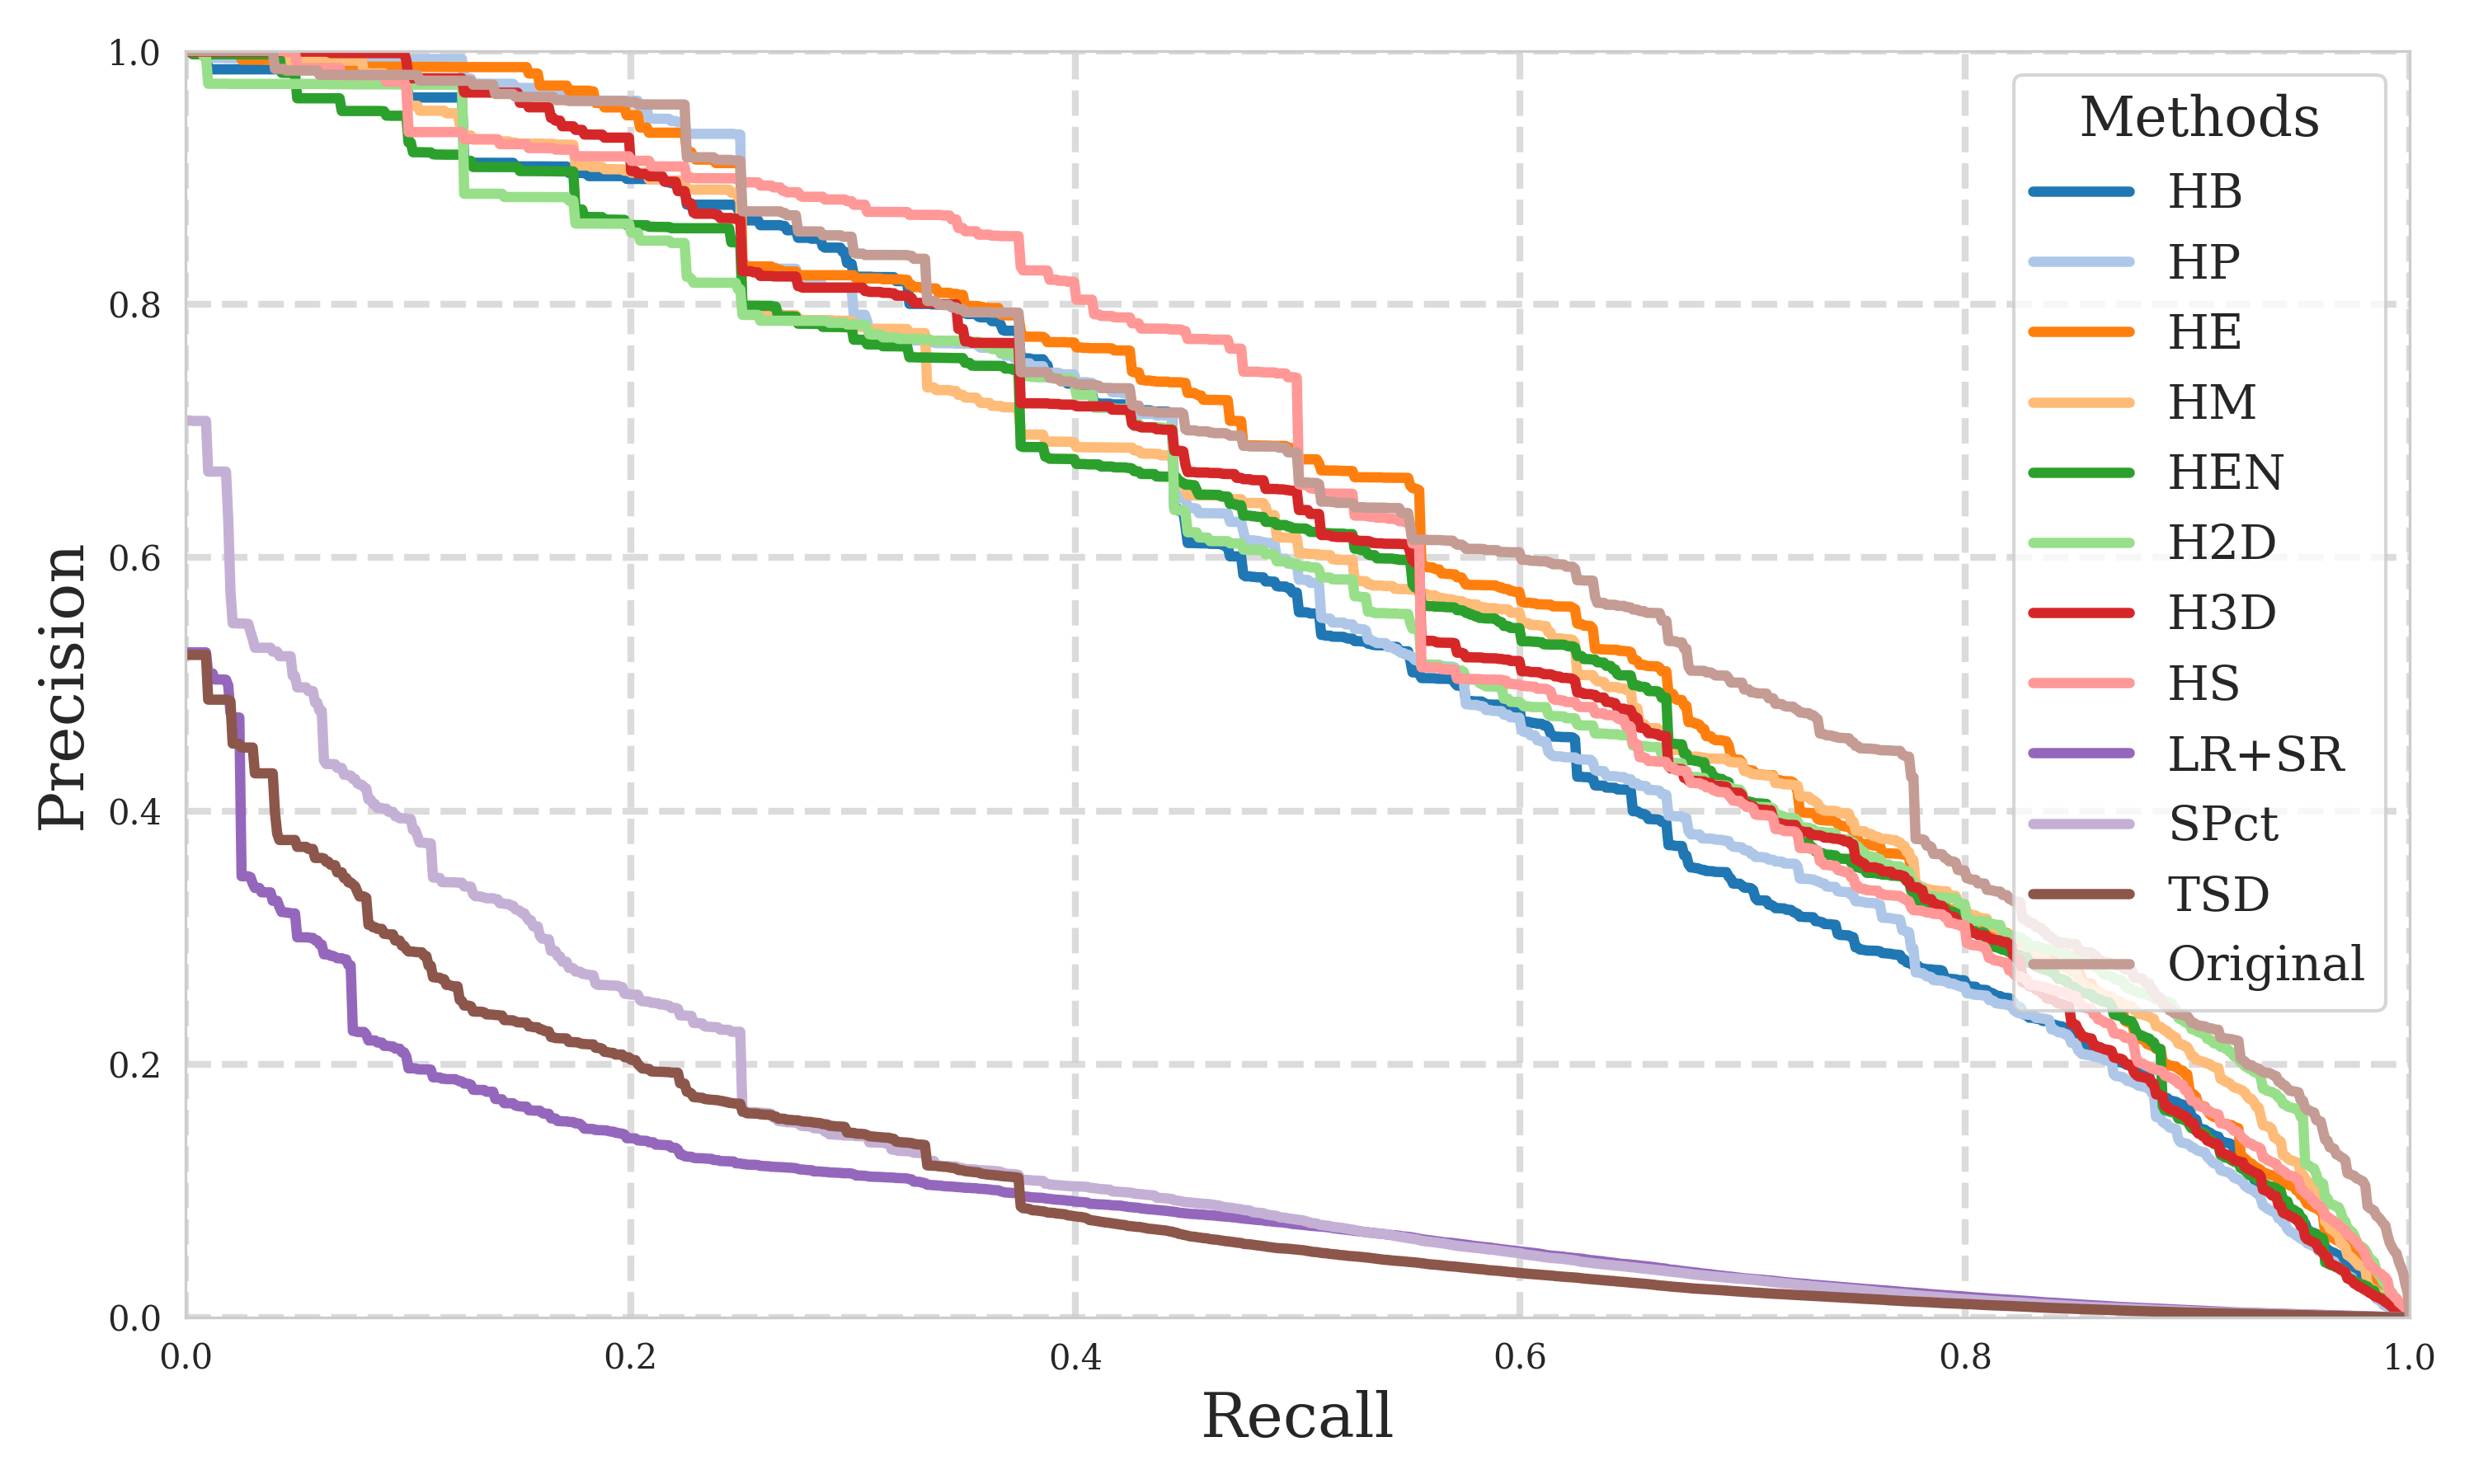}}
% \hfill
\subfloat[person]{\includegraphics[width=0.35\linewidth]{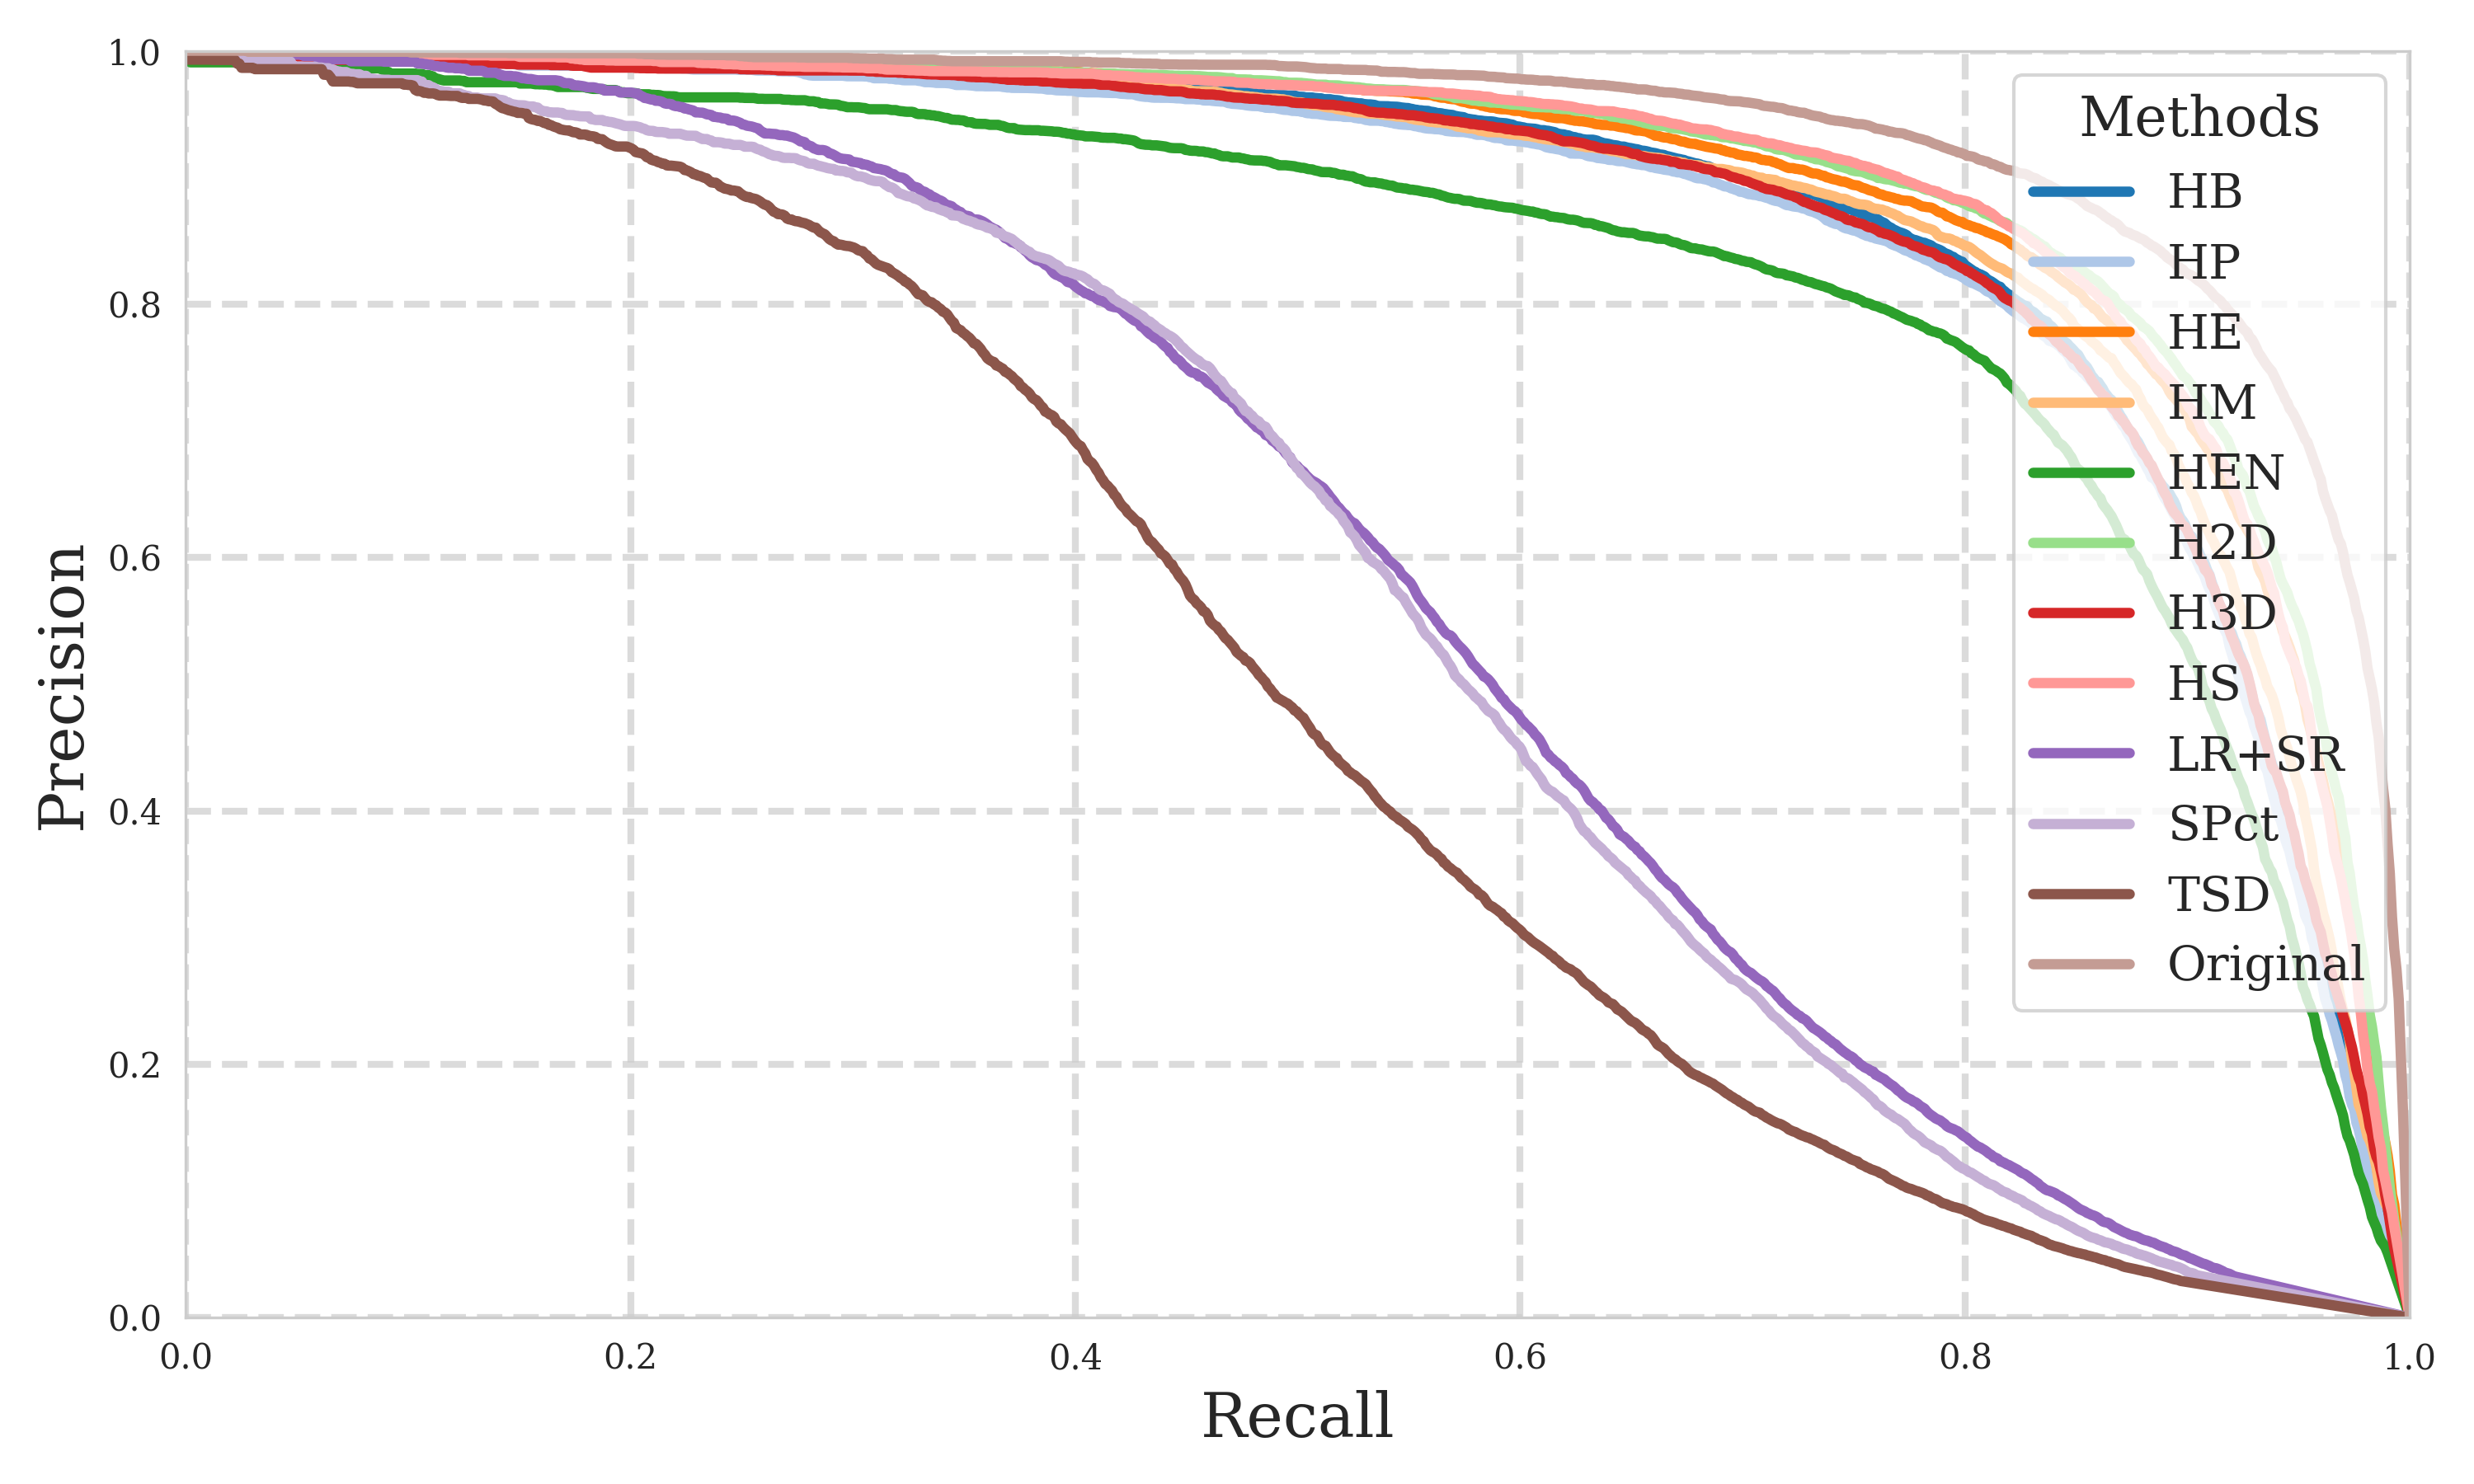}}
% \hfill
\subfloat[bicycle]{\includegraphics[width=0.35\linewidth]{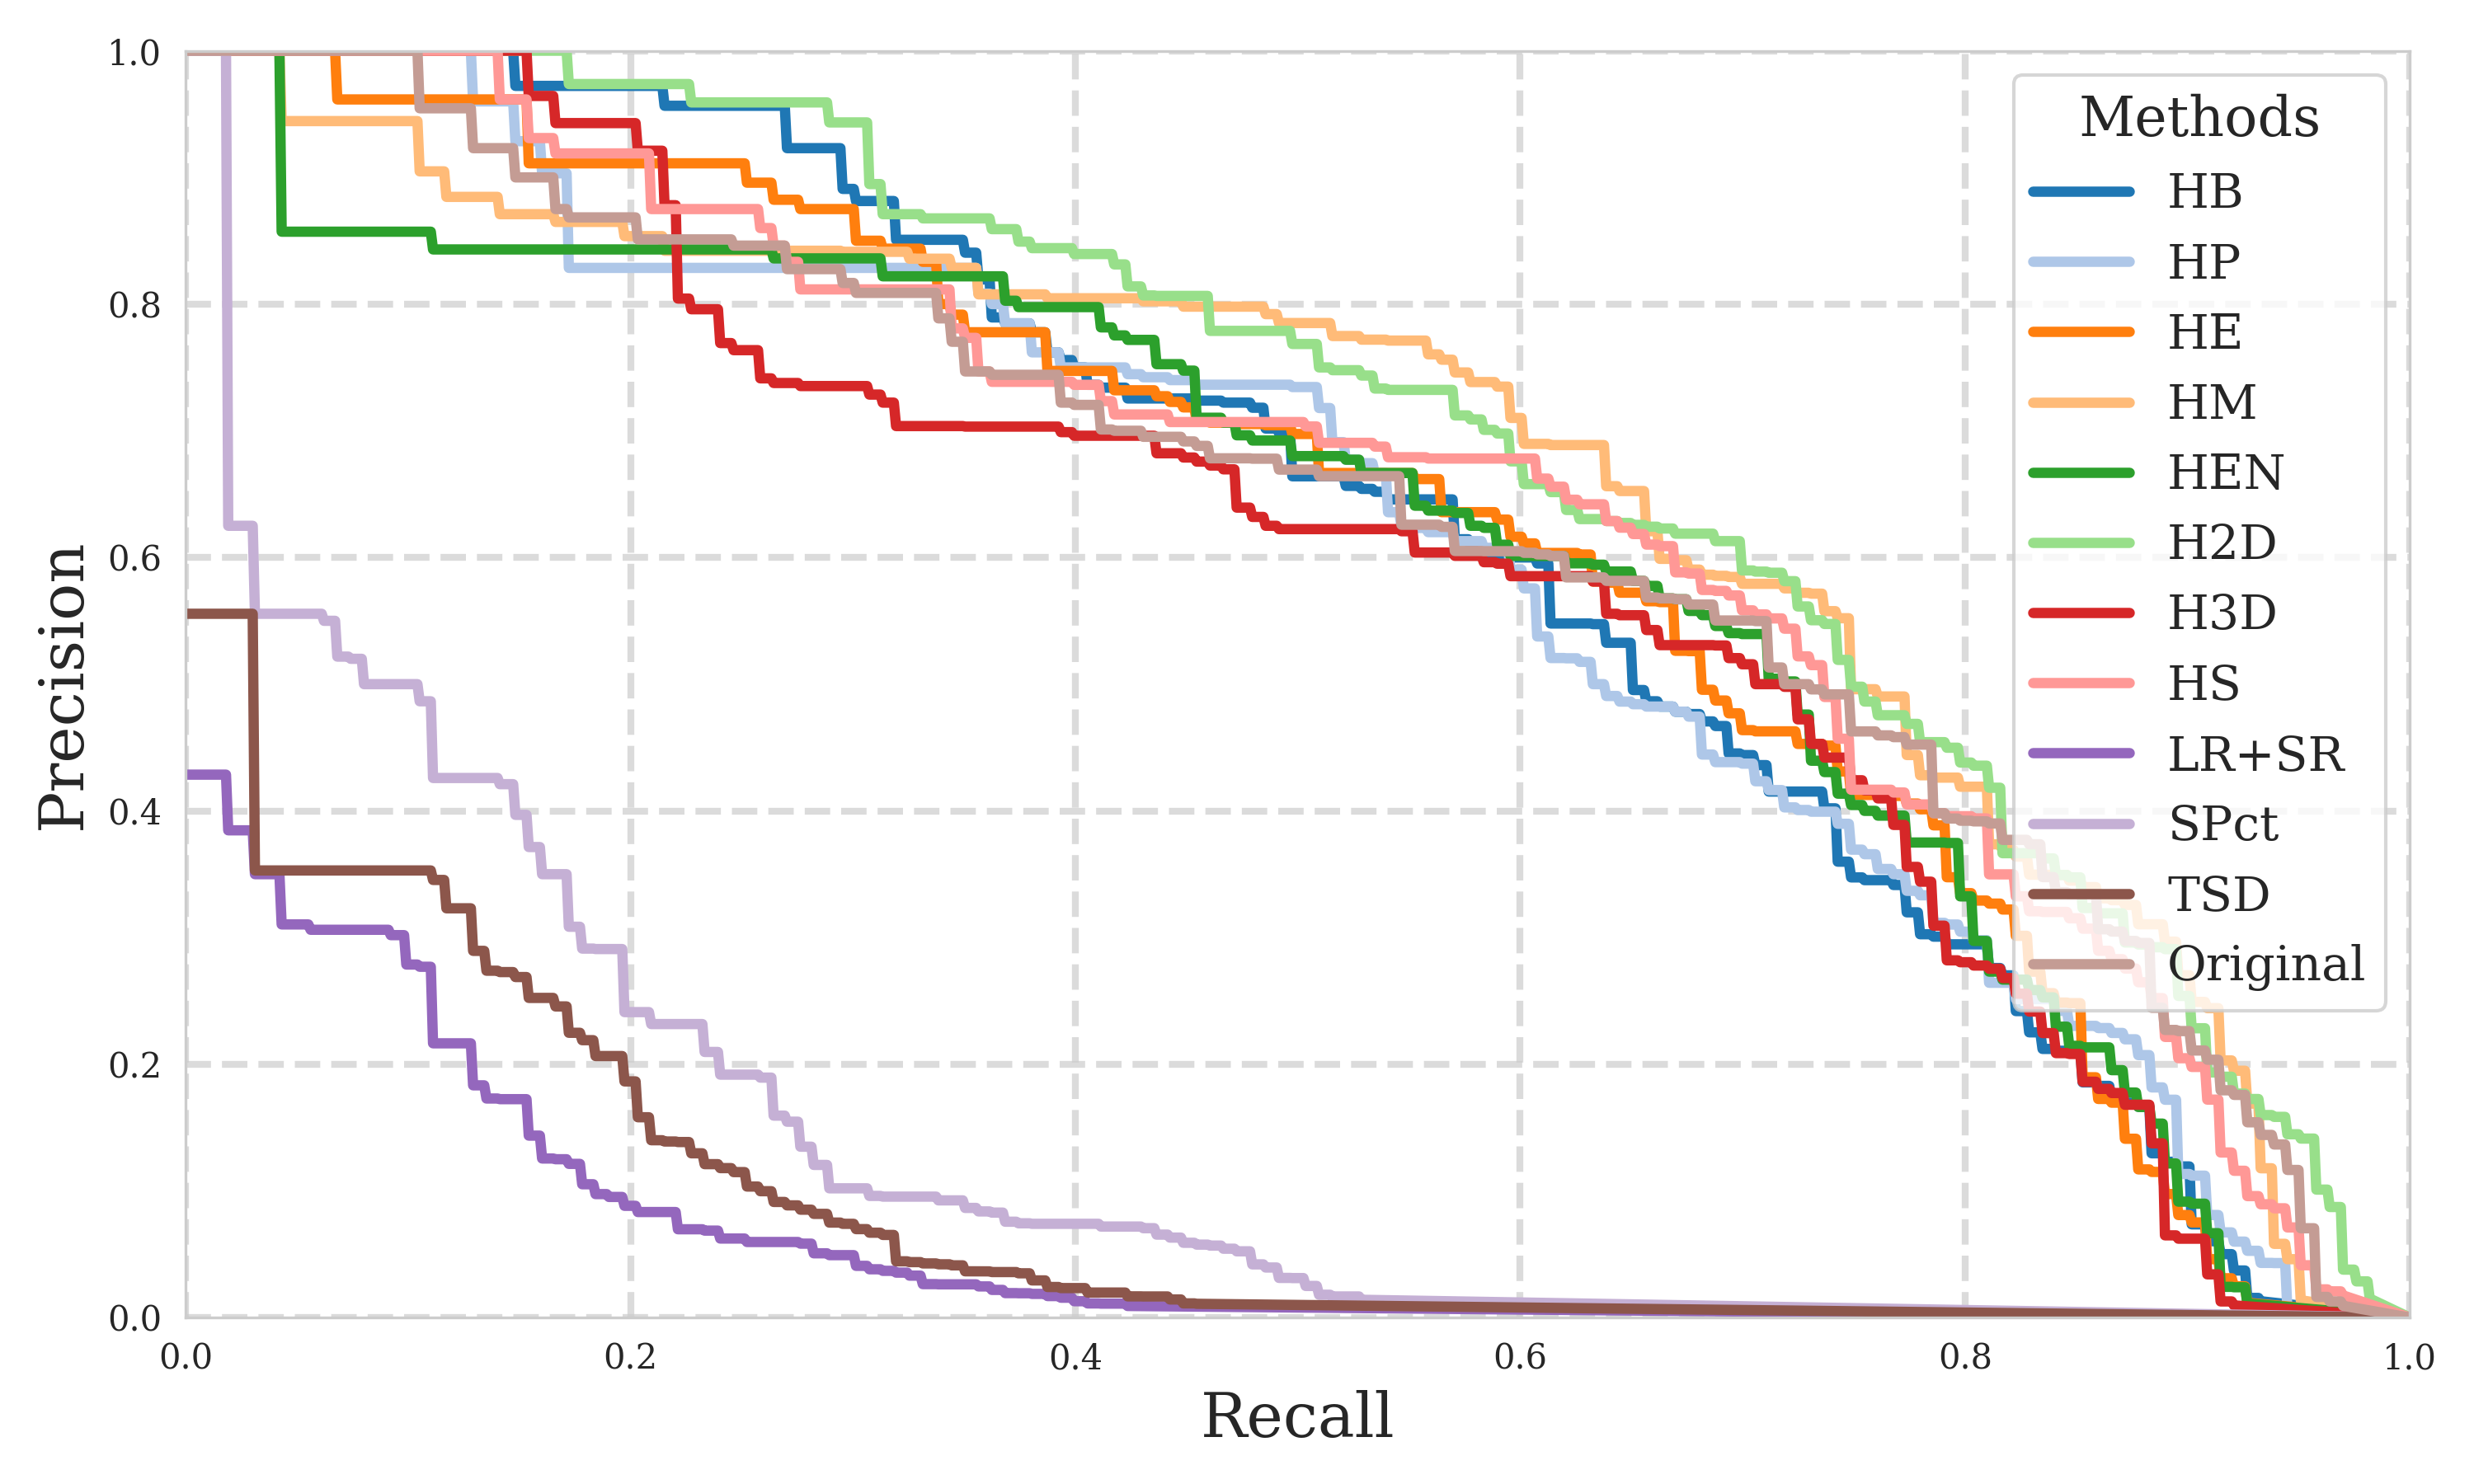}}

\subfloat[car]{ \includegraphics[width=0.35\linewidth]{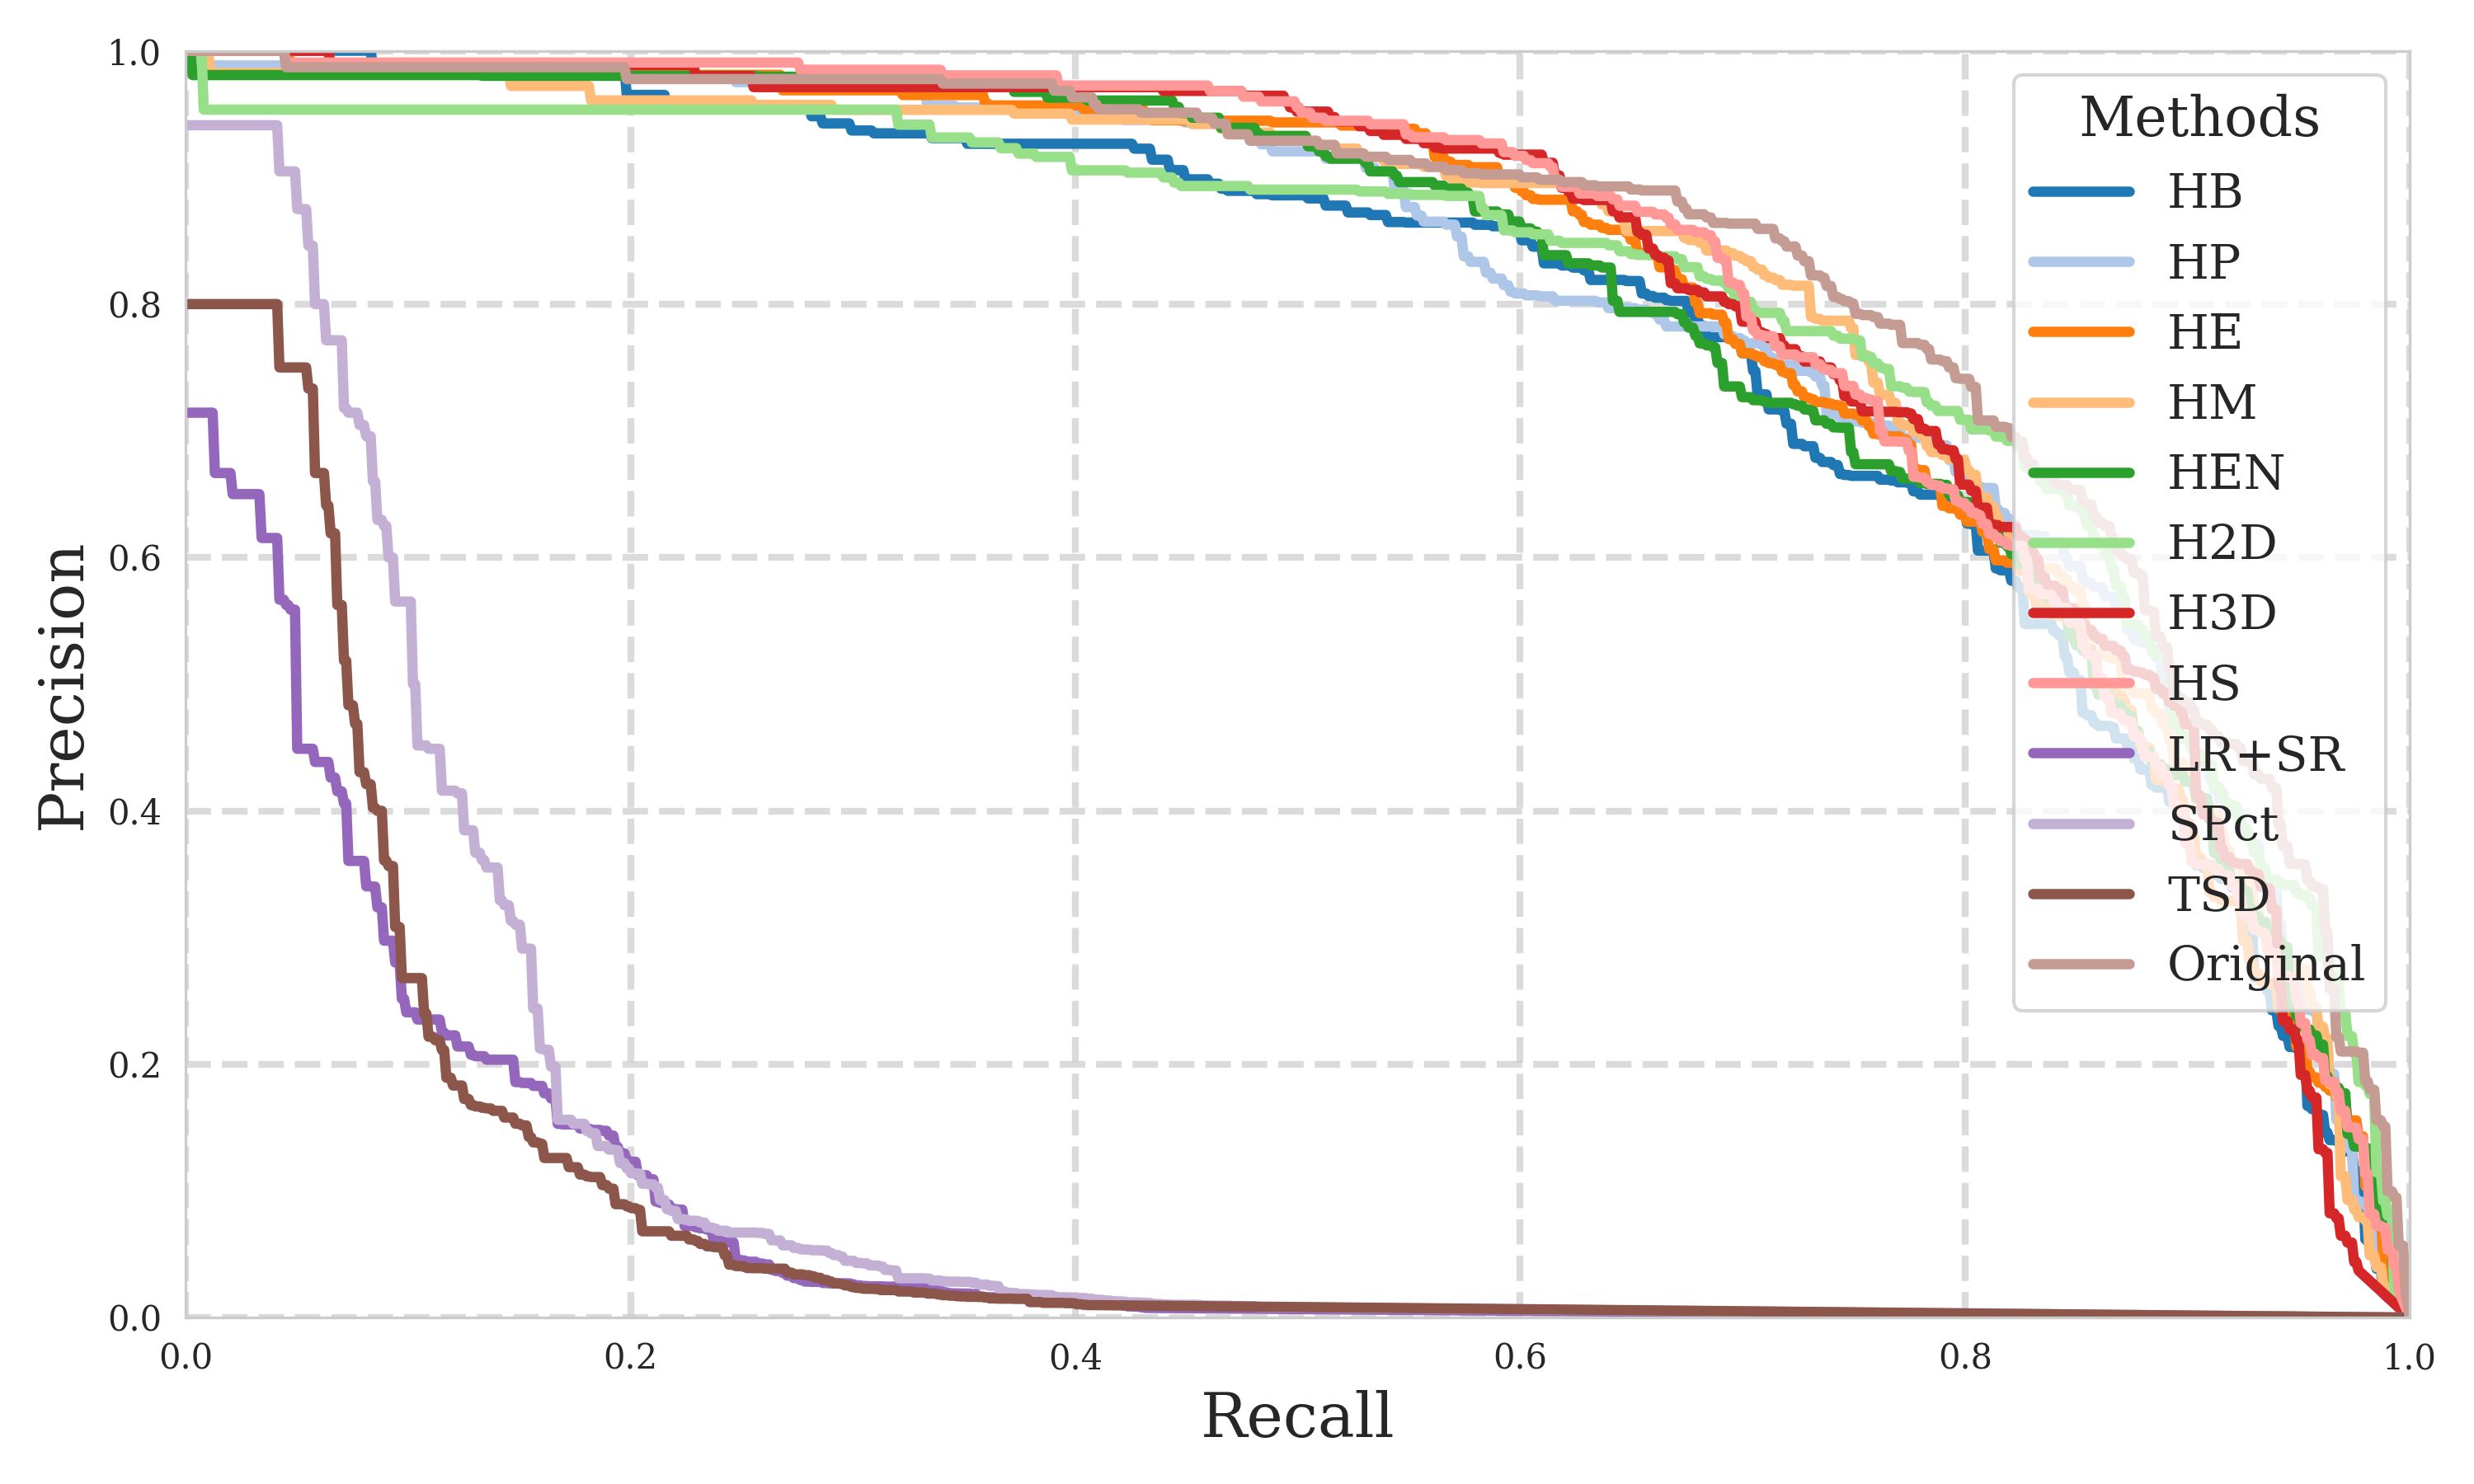}}
% \hfill
\subfloat[motorcycle]{\includegraphics[width=0.35\linewidth]{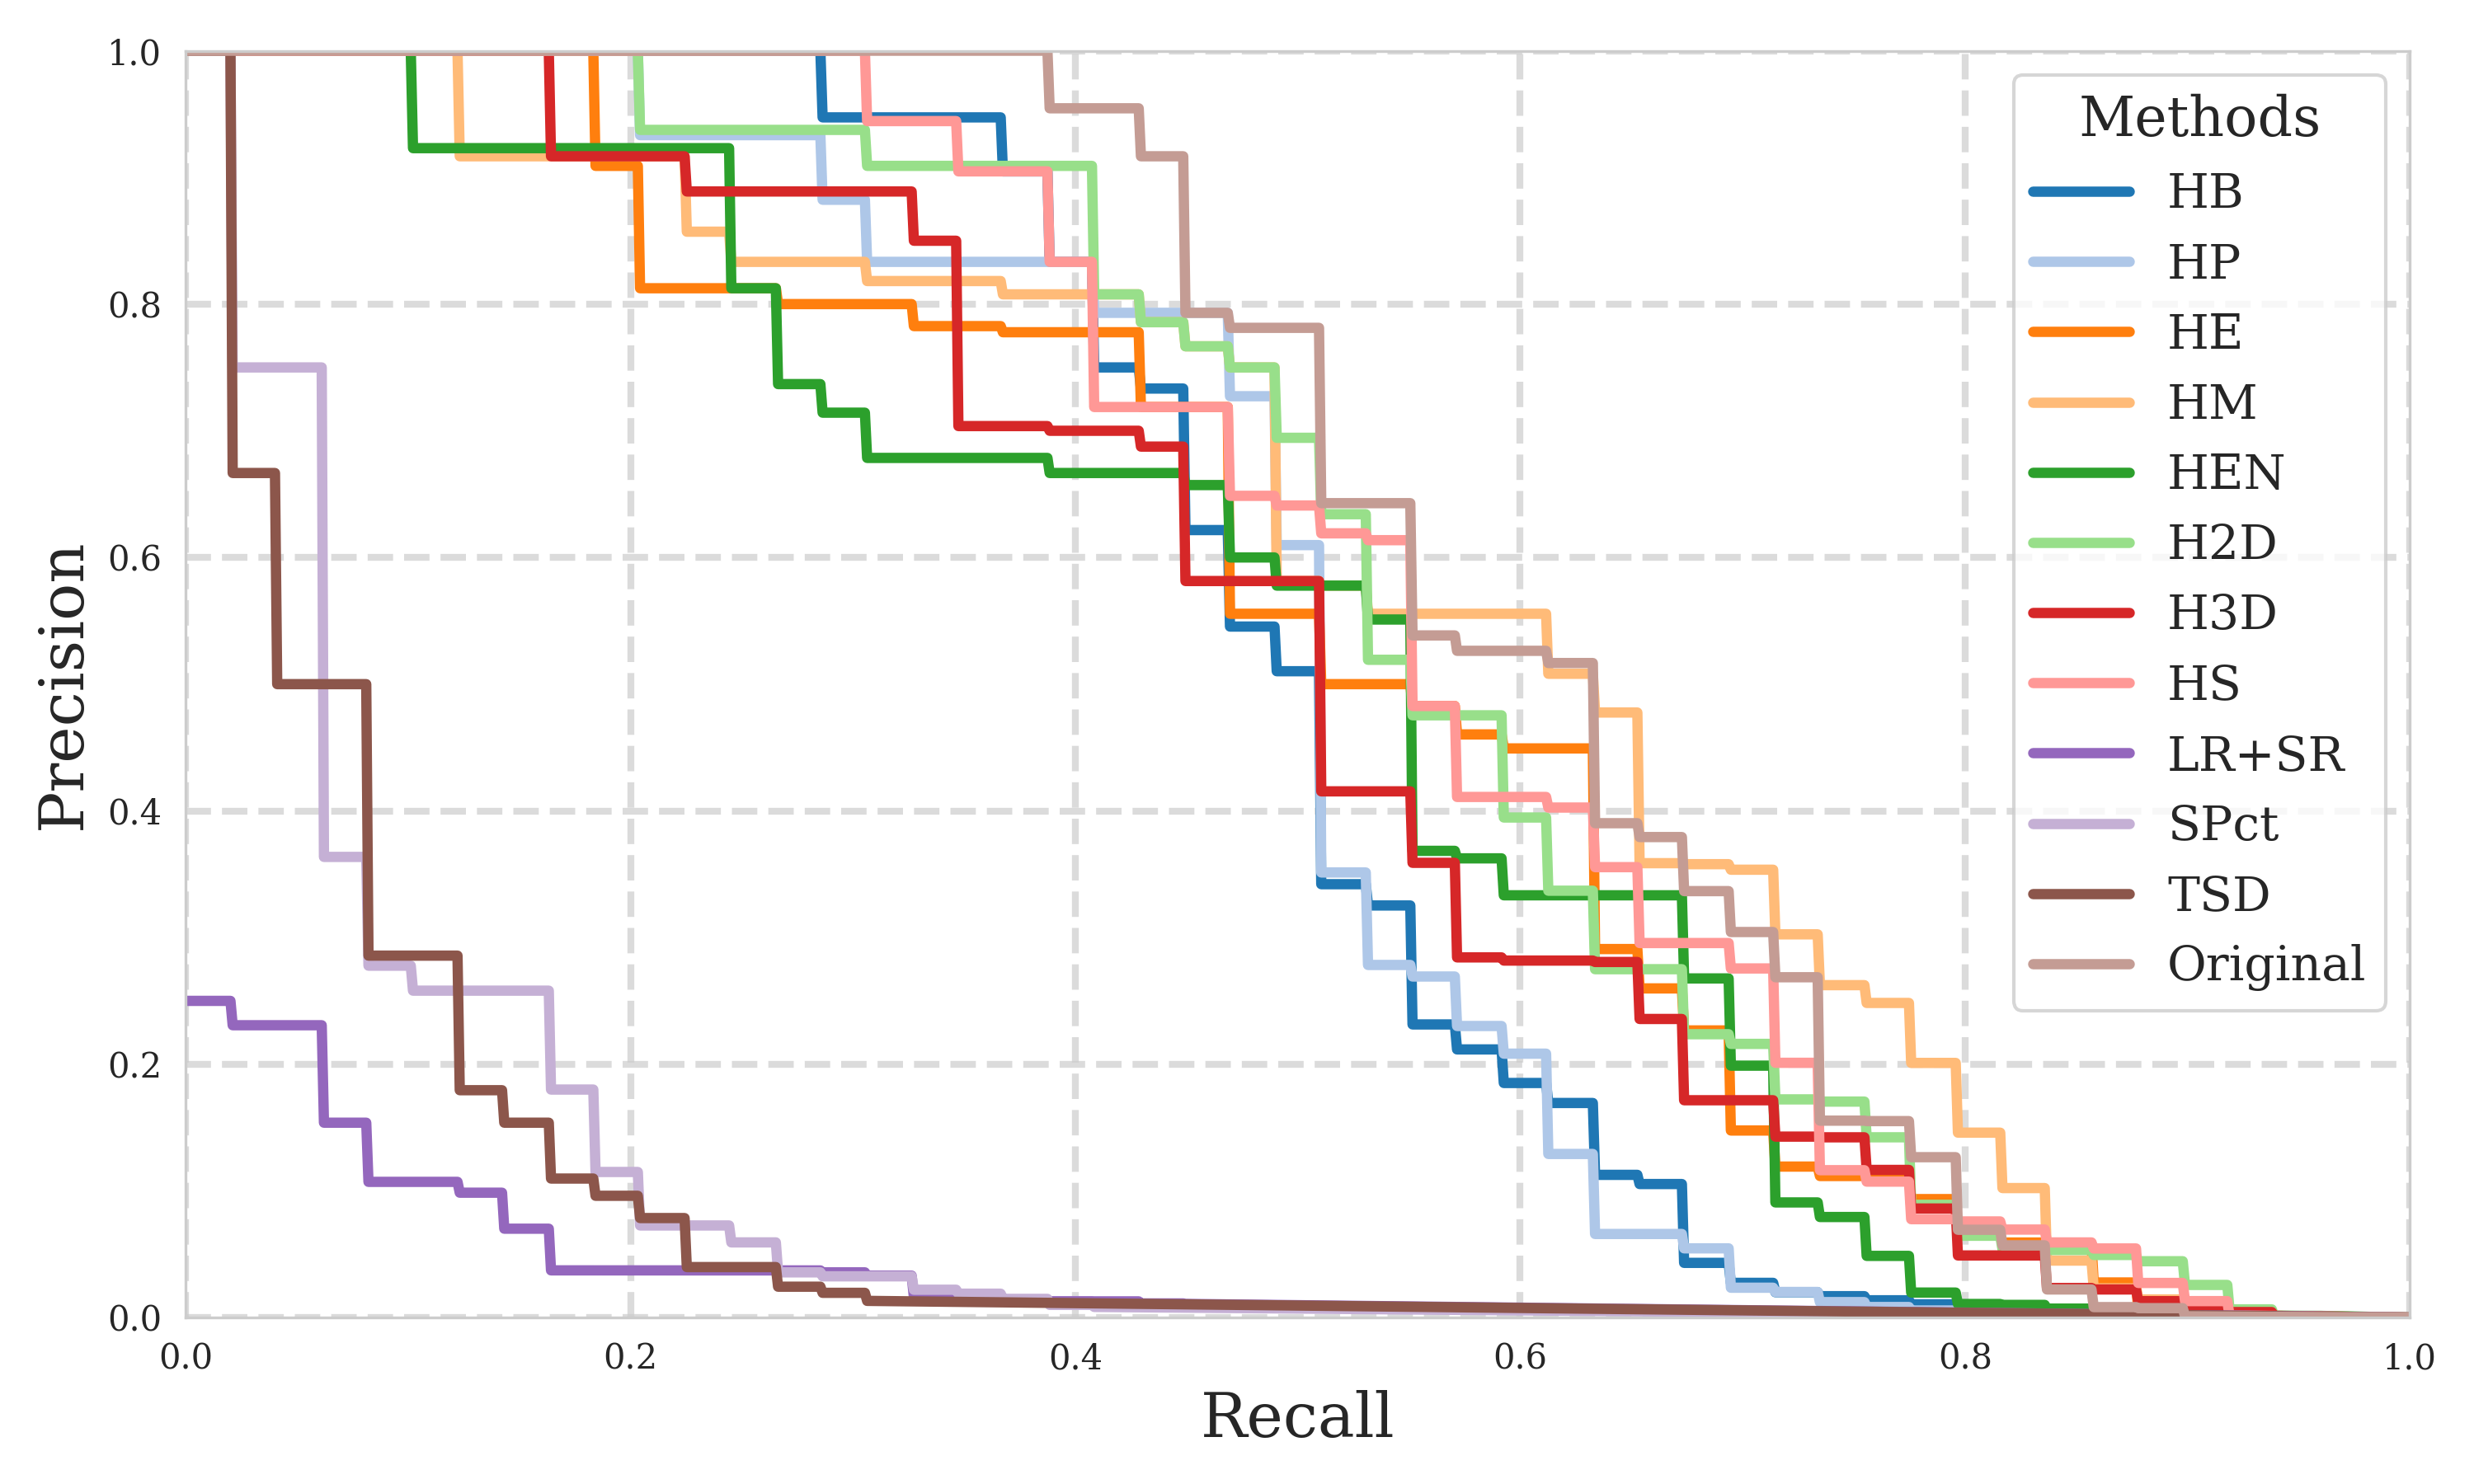}}
% \hfill
\subfloat[airplane]{\includegraphics[width=0.35\linewidth]{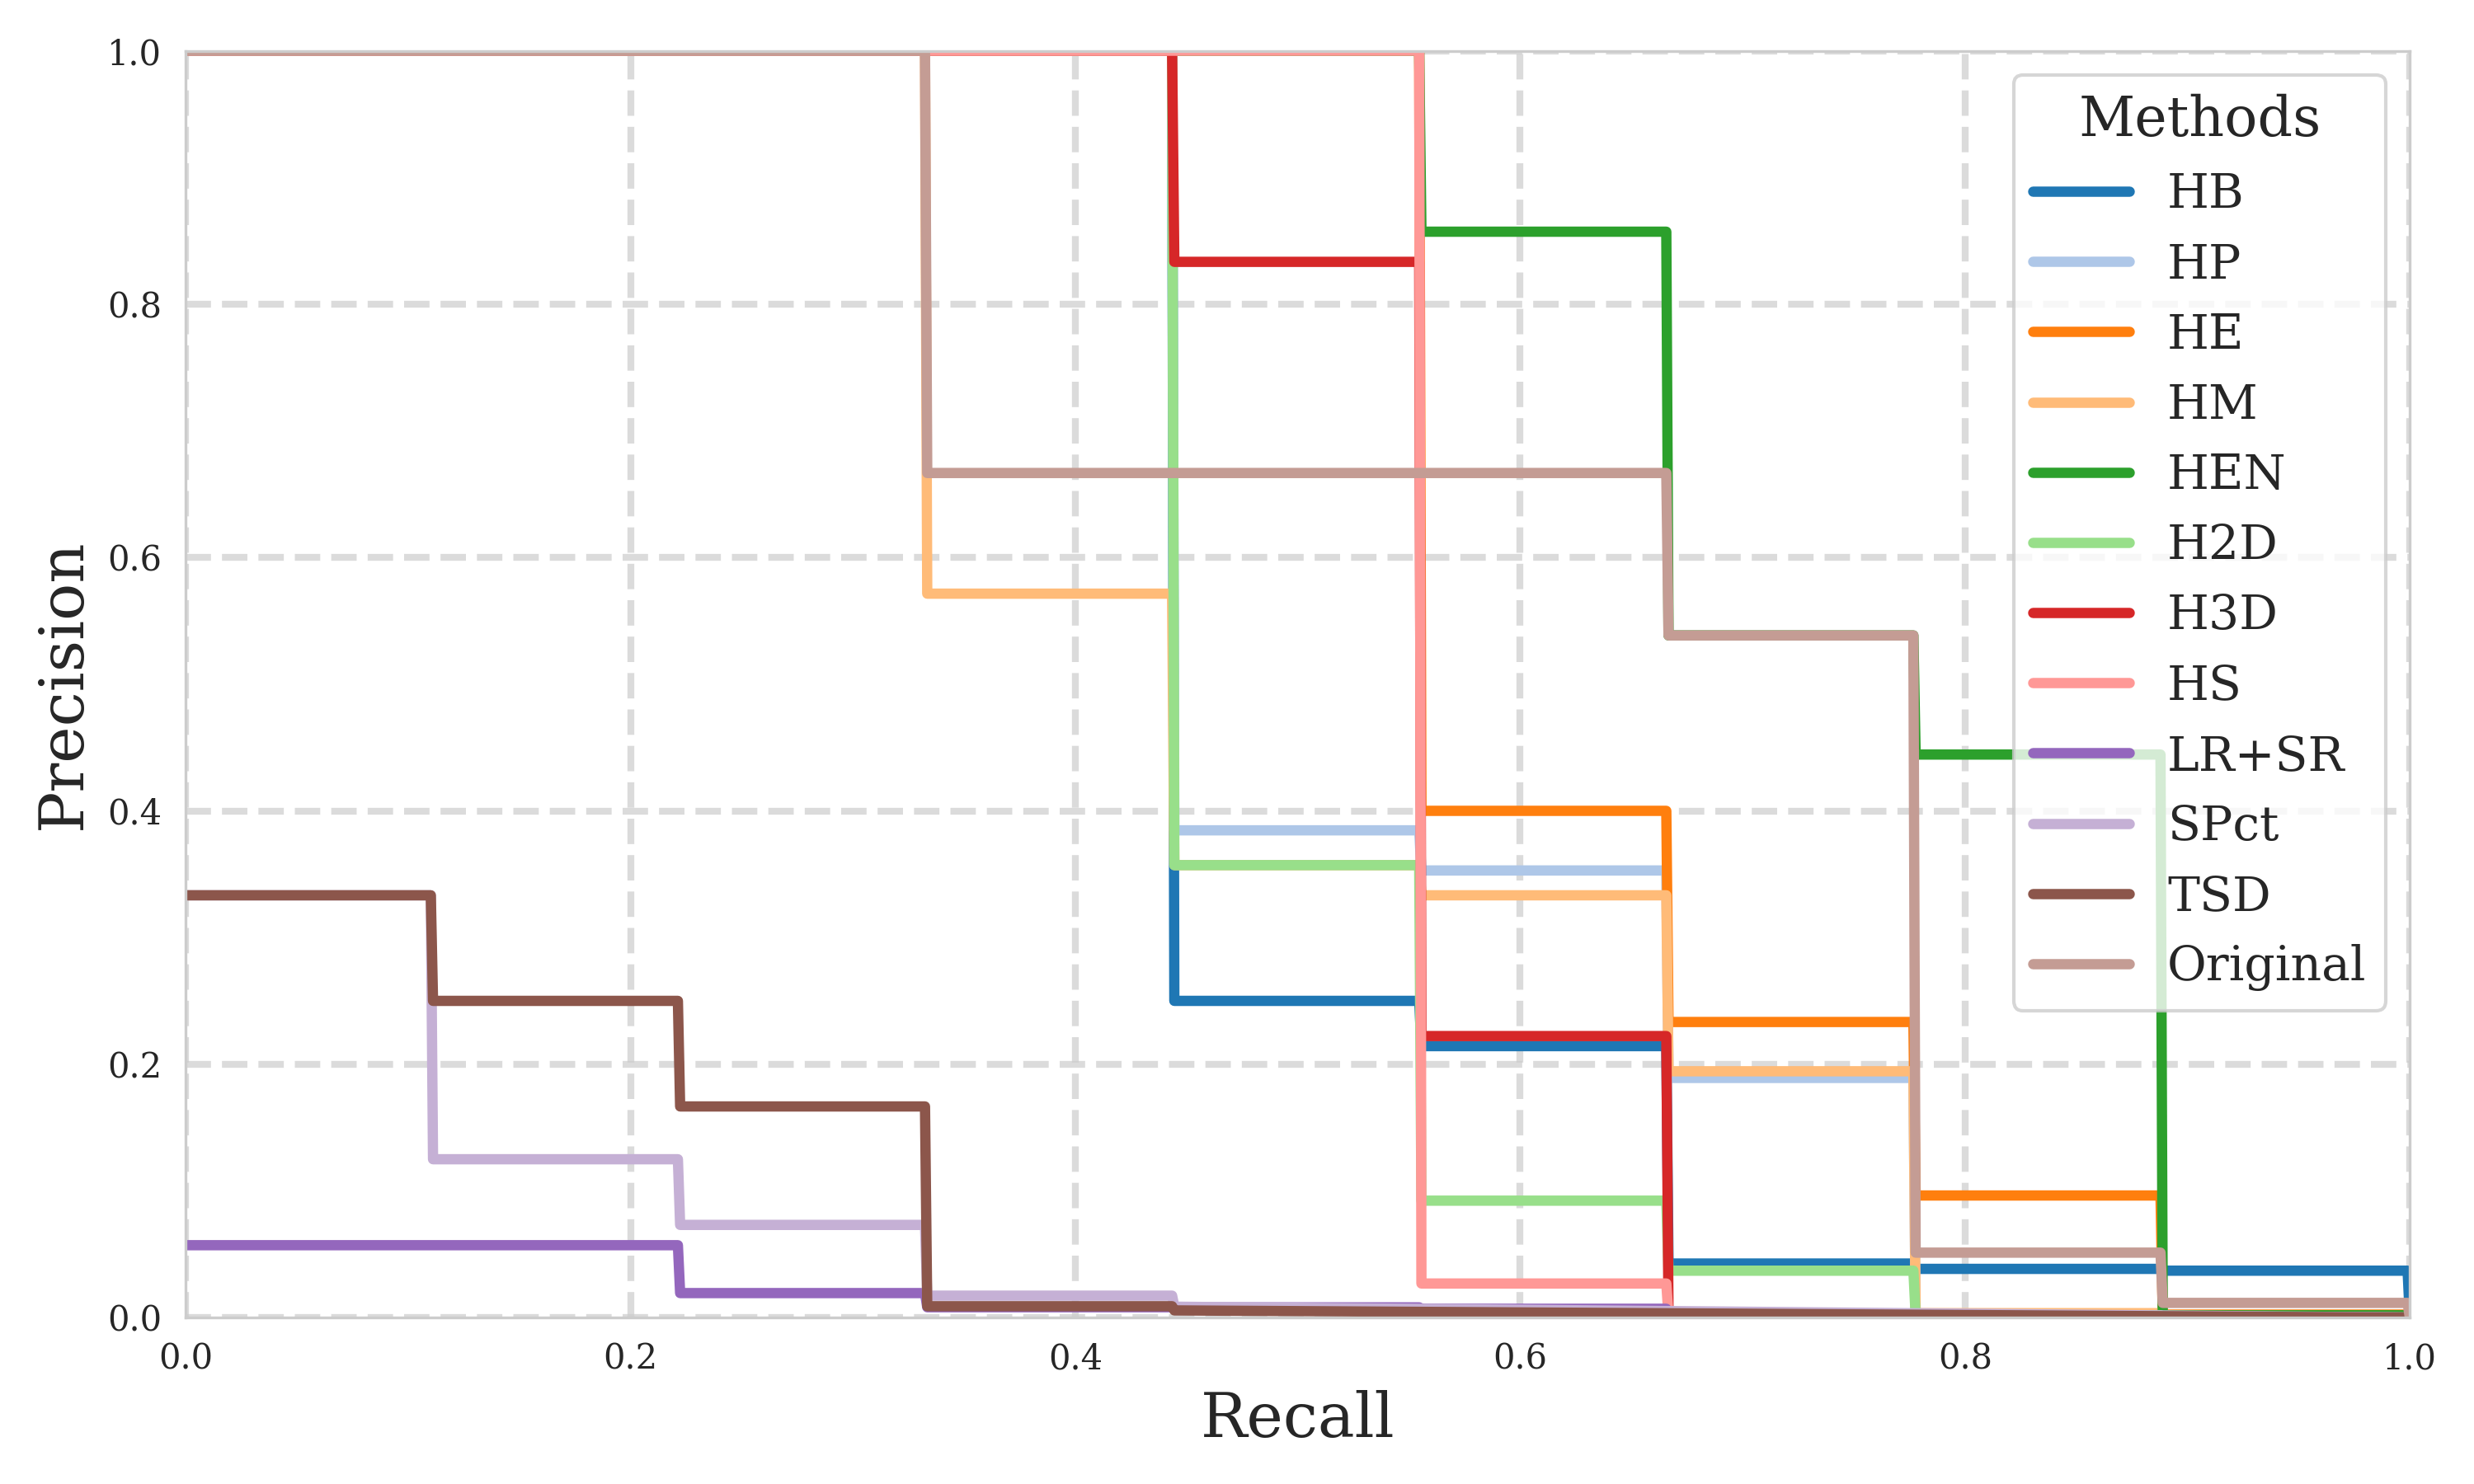}}

\subfloat[bus]{ \includegraphics[width=0.35\linewidth]{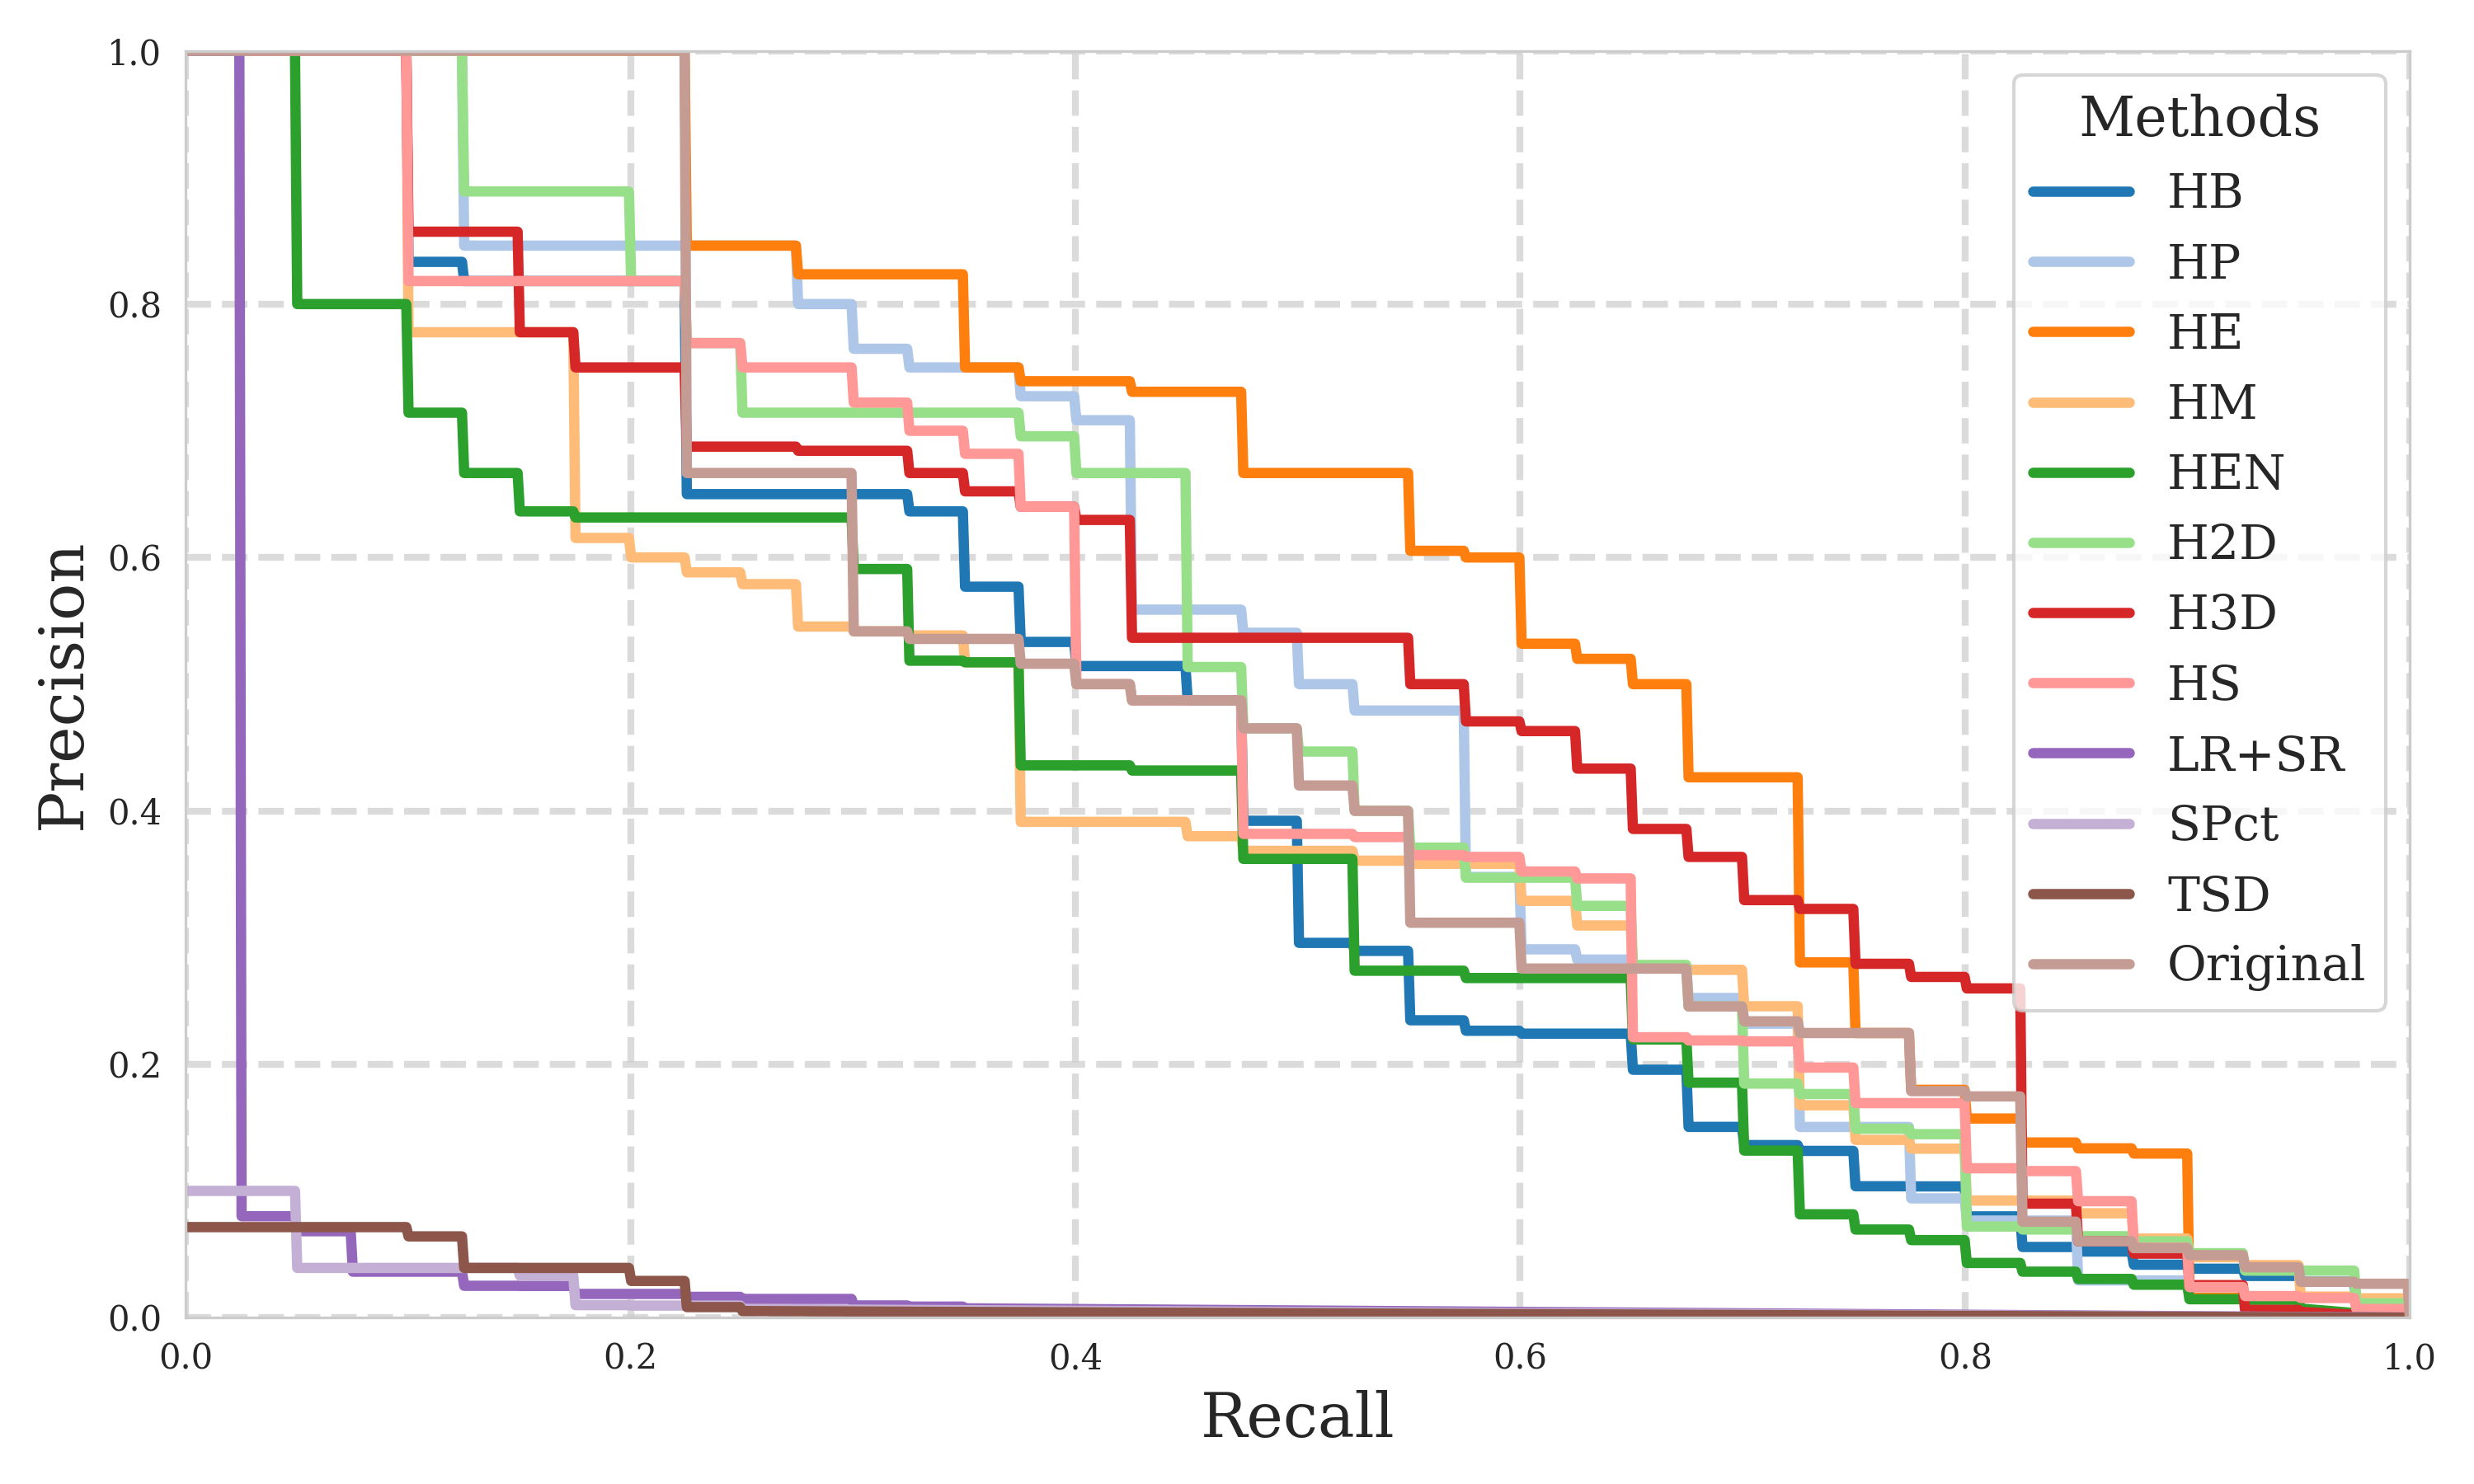}}
% \hfill
\subfloat[train]{\includegraphics[width=0.35\linewidth]{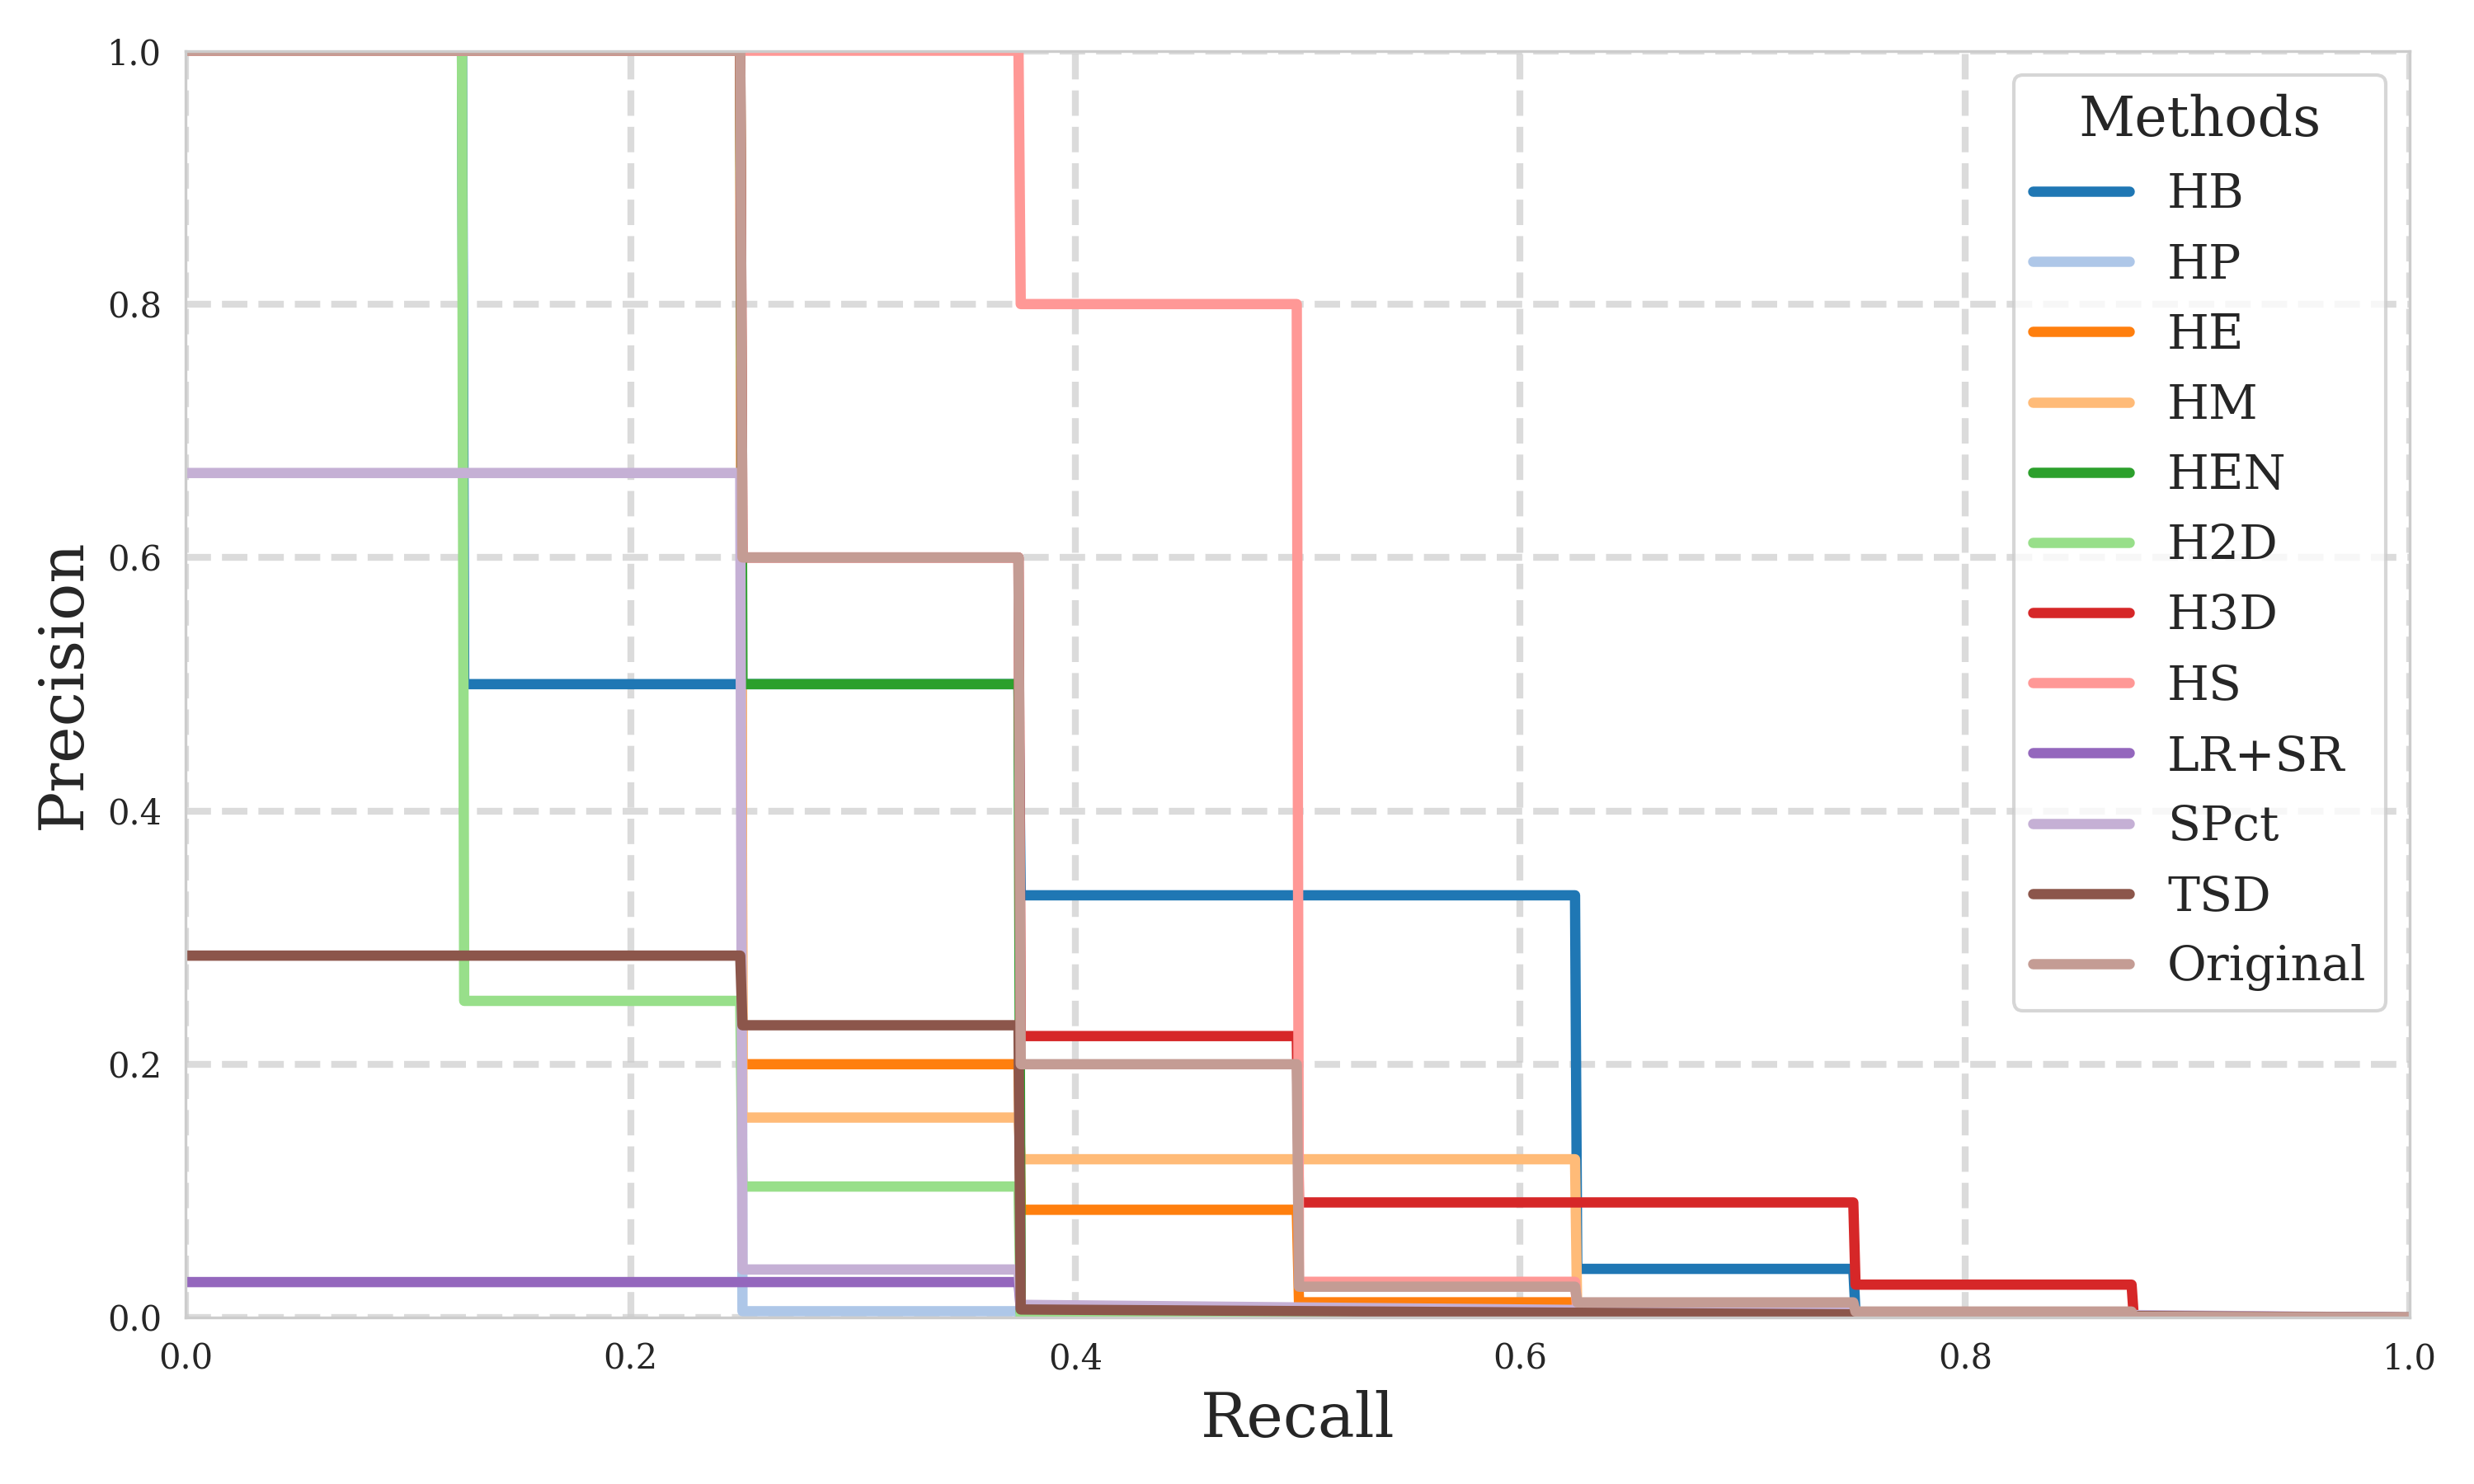}}
% \hfill
\subfloat[truck]{\includegraphics[width=0.35\linewidth]{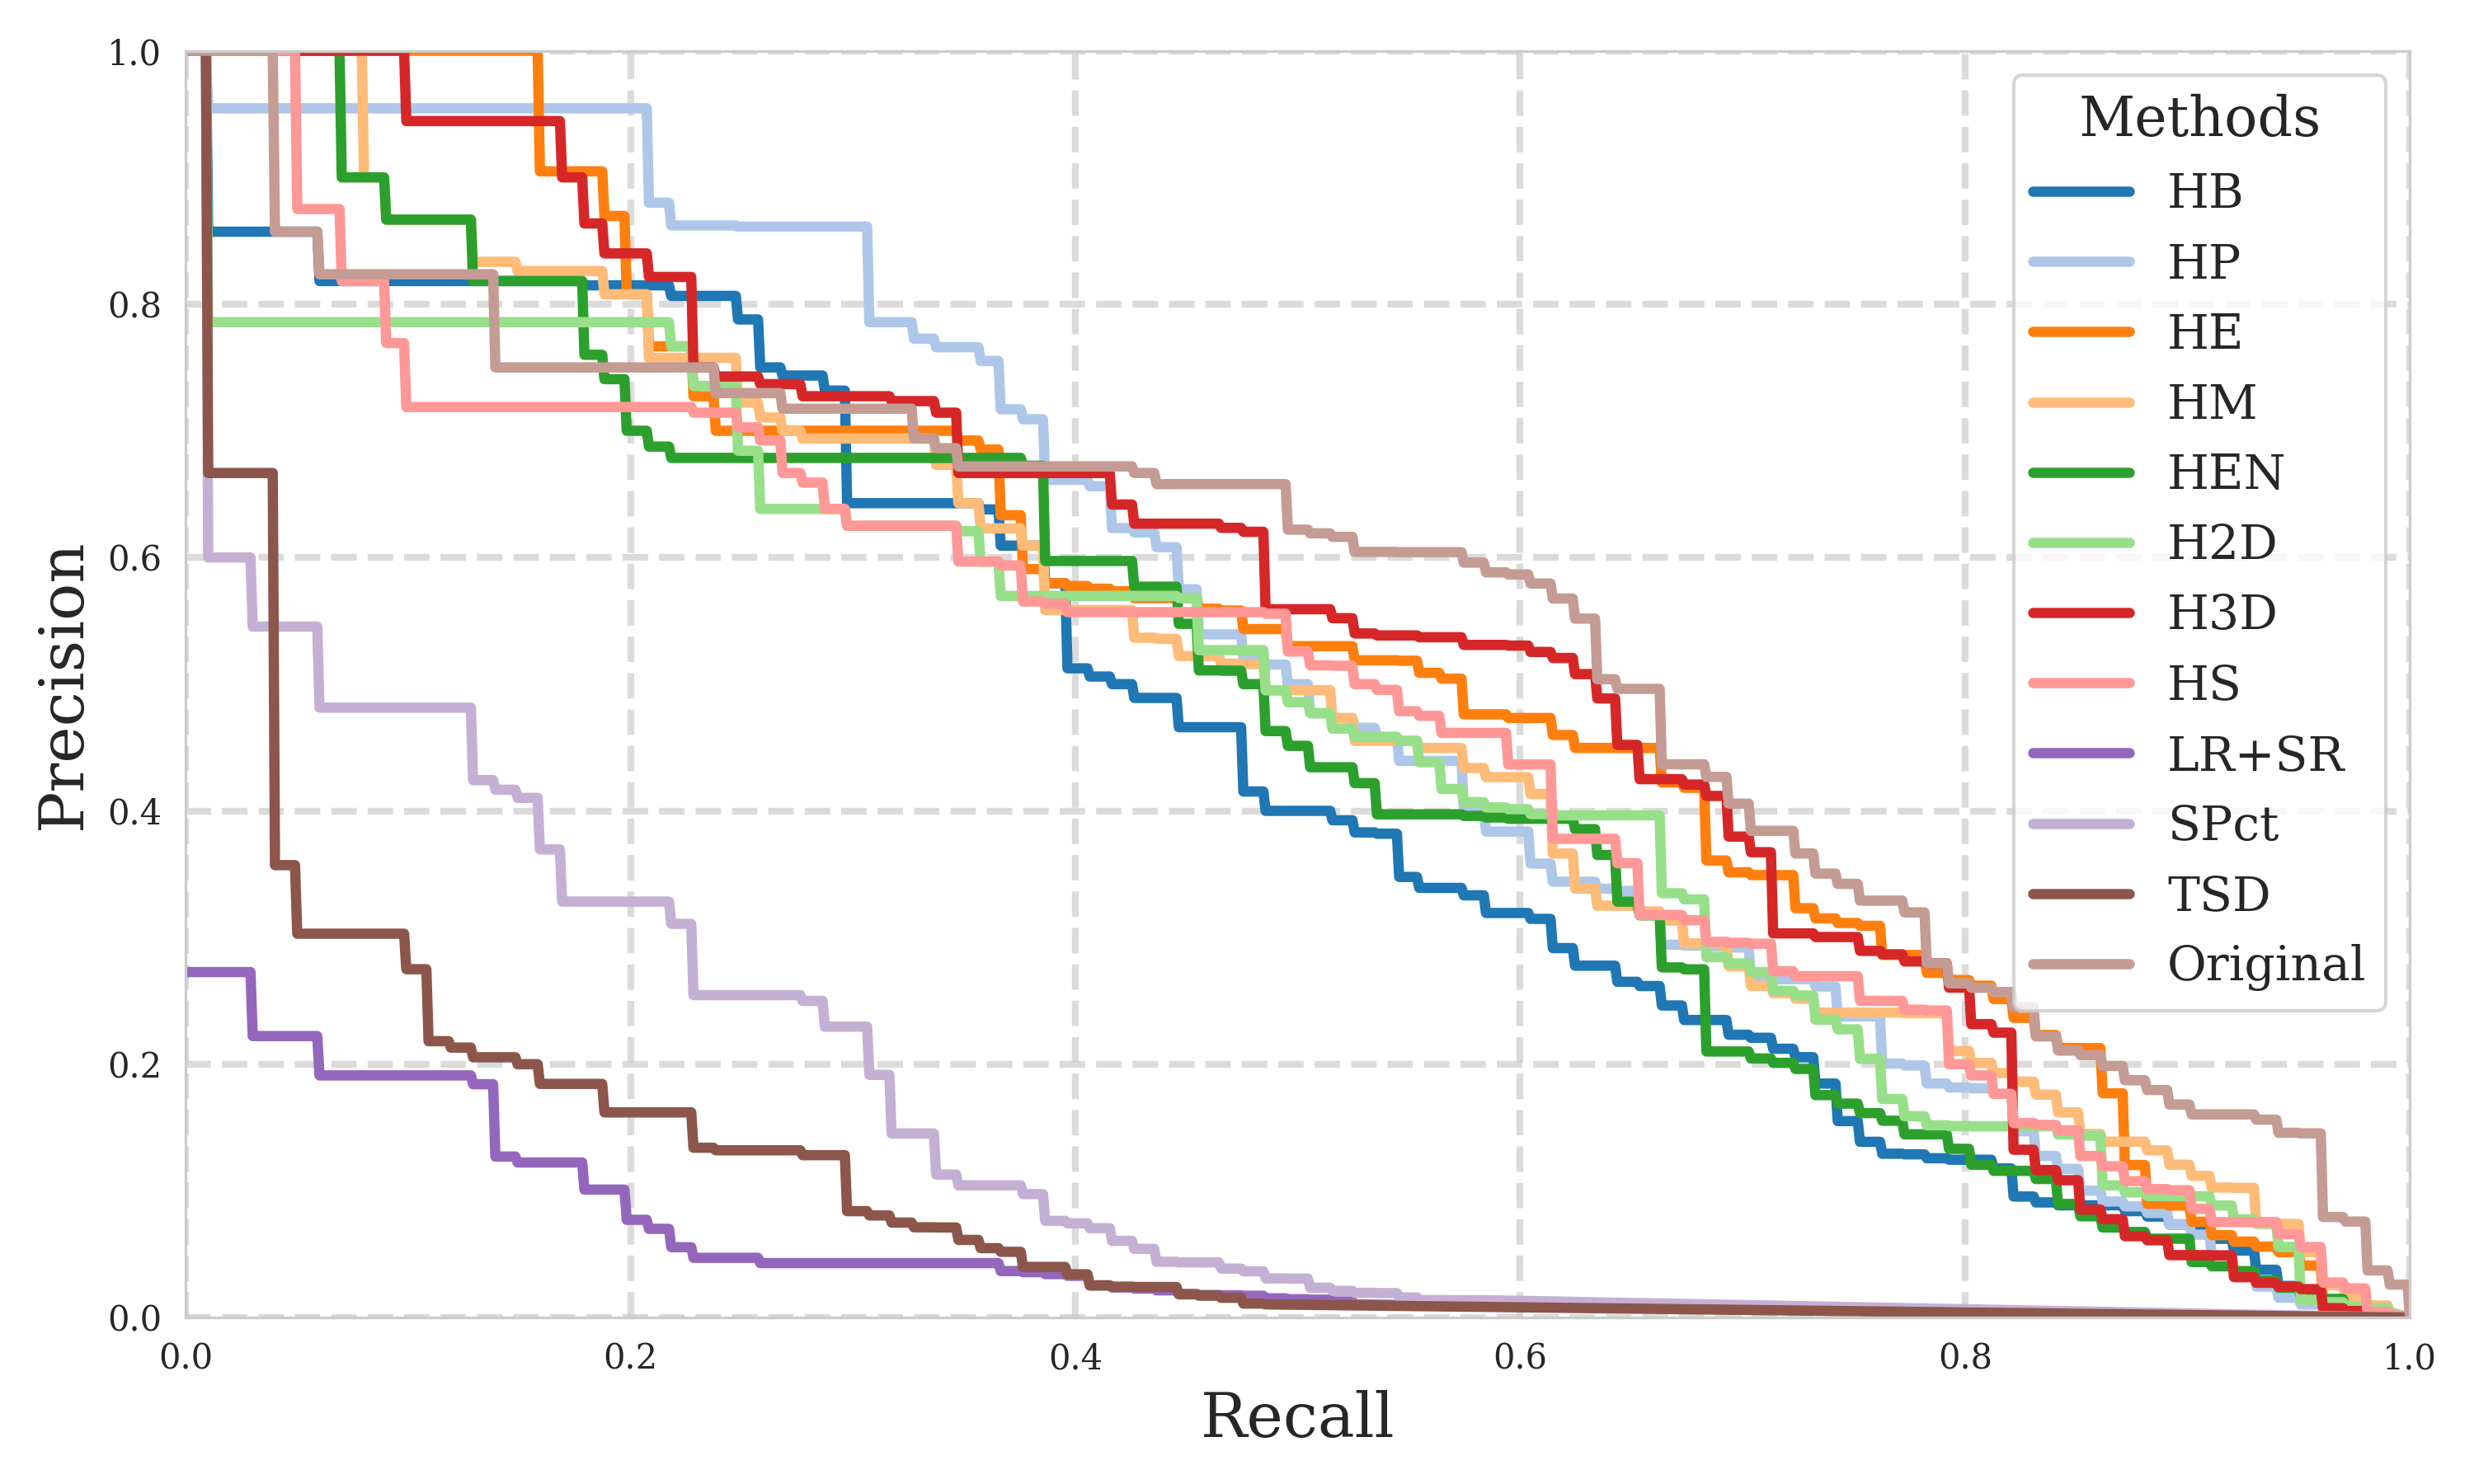}}

\subfloat[boat]{ \includegraphics[width=0.35\linewidth]{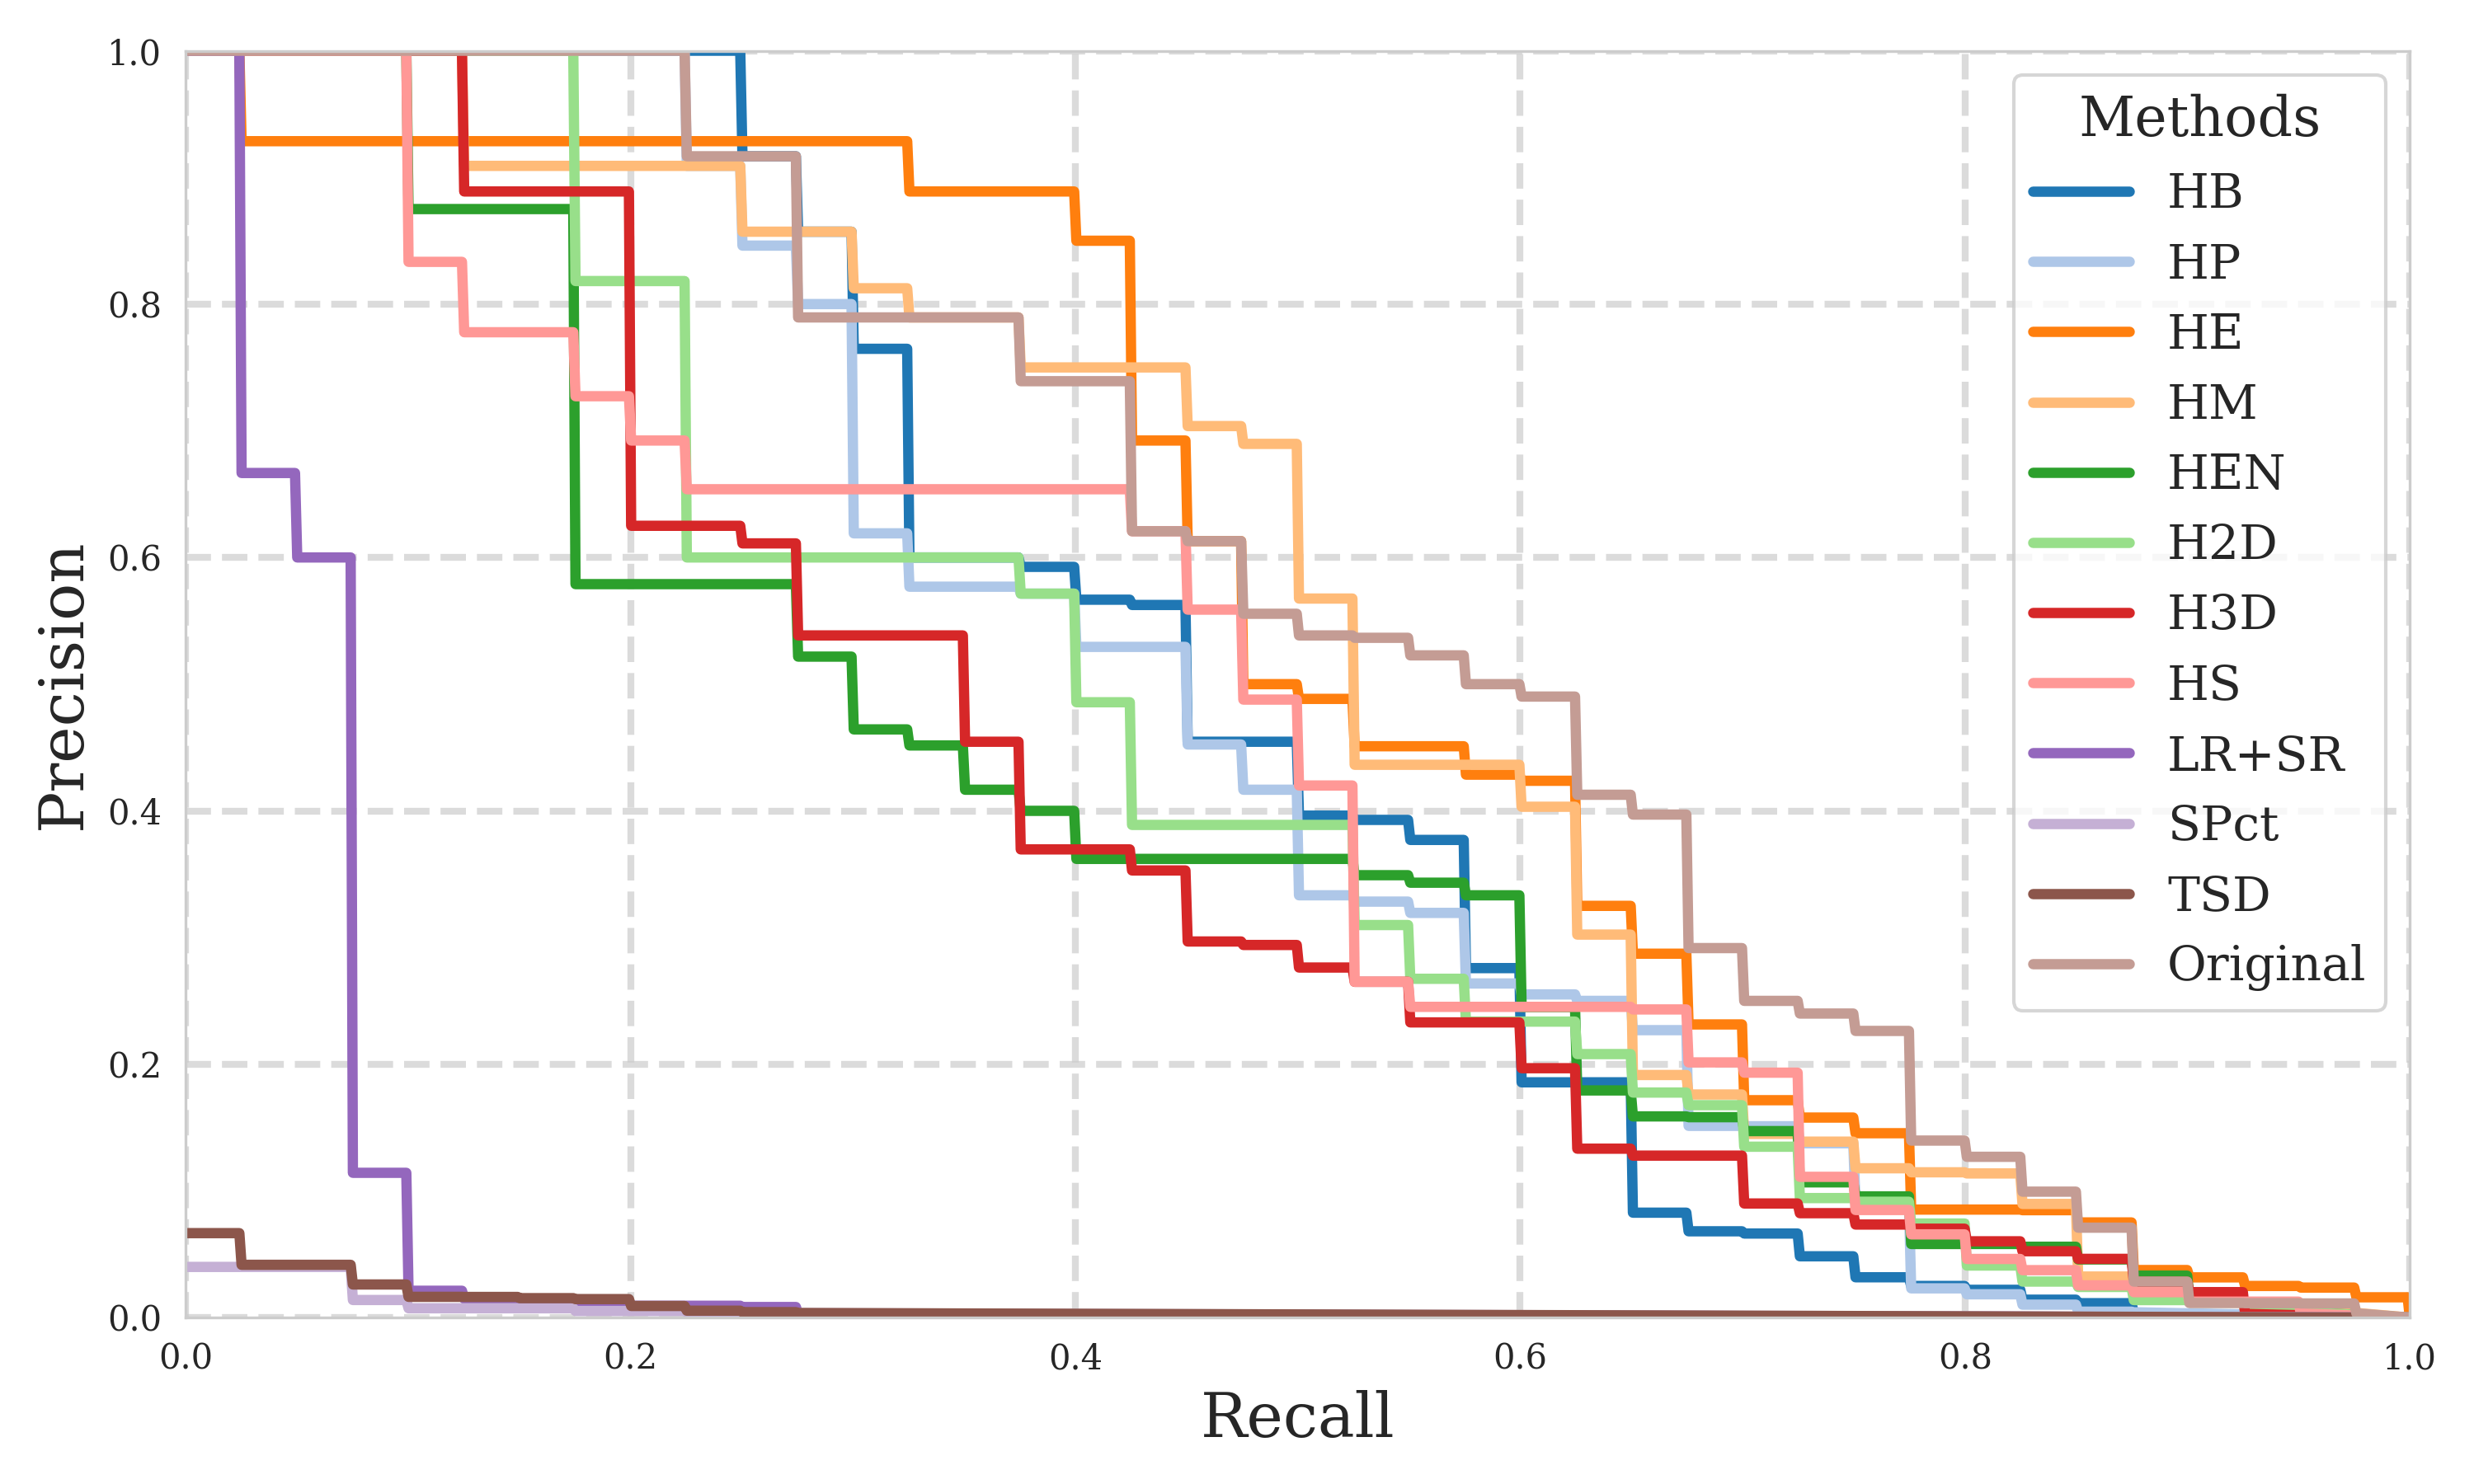}}
% \hfill
\subfloat[traffic light]{\includegraphics[width=0.35\linewidth]{figures/hrvispr_pr_curve_traffic light.png}}

\caption{Precision-Recall curves for all utility classes of HR-VISPR. }
\label{fig:pr_curves}
\end{figure*}

{
    \small
    \bibliographystyle{ieeenat_fullname}
    \bibliography{references}
}
% \putbib[references]
